# Supplementary material for: SMURF: Continuous Dynamics for Motion-Deblurring Radiance Fields
Source: arXiv:2403.07547 source file (2025-05-15)
Supplement: Supplementary file 1 [file X_suppl.tex]

\clearpage
\setcounter{page}{1}
%\maketitlesupplementary

\twocolumn[{
		\renewcommand\twocolumn[1][]{#1}
		\maketitlesupplementary
		\begin{center}
				\centering
				\captionsetup{type=figure}
%				\vspace{-6mm}
				\includegraphics[width=1\linewidth]{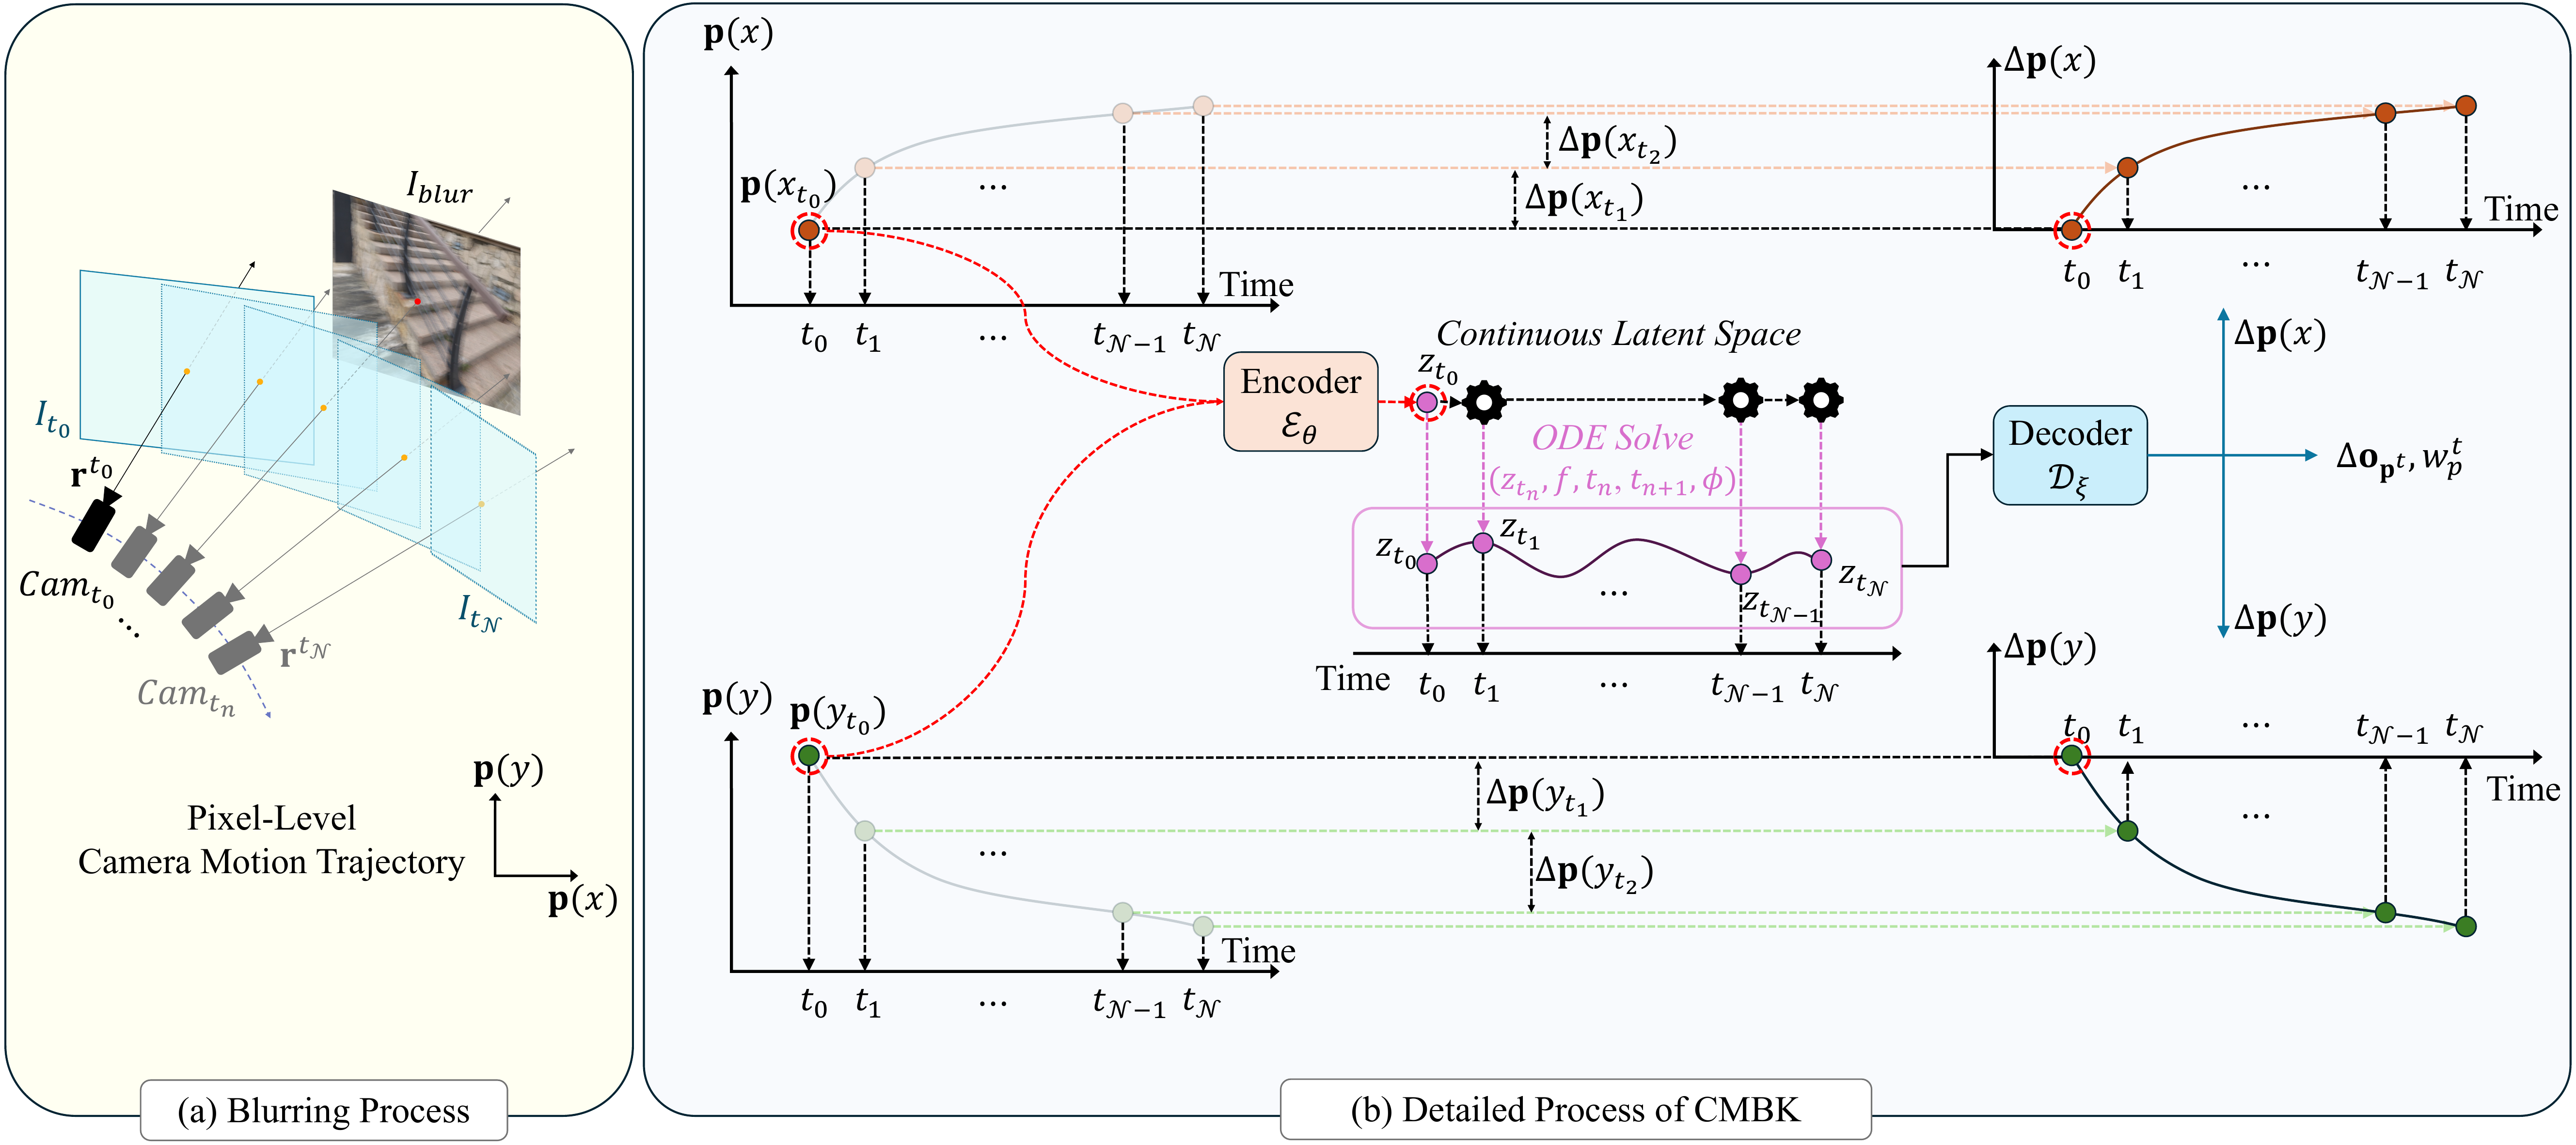}
				\caption{\textbf{Detailed process for generating kernel}. To highlight the continuous dynamics in the latent space, all embedding functions are omitted from the figure. $\mathbf{p}(x_{t_{0}})$ and $\mathbf{p}(y_{t_{0}})$ correspond to the $x$ and $y$ coordinates of the pixel associated with the initial ray, respectively.}
				\label{fig:method_overview}
%				\vspace{+4mm}
			\end{center}
	}]

%\begin{strip}
%	\centering
%	\textbf{\LARGE{Appendix of \\ \vspace{+3mm}SMURF: Continuous Dynamics for Motion-Deblurring Radiance Fields}\vspace{+13mm}}
%	\includegraphics[width=\linewidth]{figures/smurf_figure_appendix_1.pdf}
%	\captionof{figure}{\textbf{Detailed process for generating kernel}. To highlight the continuous dynamics in the latent space, all embedding functions are omitted from the figure. $\mathbf{p}(x_{t_{0}})$ and $\mathbf{p}(y_{t_{0}})$ correspond to the $x$ and $y$ coordinates of the pixel associated with the initial ray, respectively.}
%	\label{fig:method_overview}
%\end{strip}

\section{Details of CMBK}

We elaborate on the continuous dynamics of the proposed CMBK as shown in~\cref{fig:method_overview}. We assume that camera motion encompasses inherent dynamics with a unique solution. The assumed solution is represented by the lighter circles in the left plots of~\cref{fig:method_overview} (b). Rather than implementing the inherent dynamics in a simple physical space, we refine them within a latent space with parametric learning. The continuous dynamics of CMBK involve transforming the pixel coordinates corresponding to the ray into latent features via a parameterized encoder $\mathcal{E}_{\theta}$, and a unique numerical solution~\cite{lindelof1894application} is obtained by solving the initial value problem on the latent space through a neural ordinary differential equation~\cite{chen2018neural}. The solution in the latent space is transformed to the physical space by the decoder $\mathcal{D}_{\xi}$, which represents the change in ray origin, corresponding weight, and the change in pixel of the warped ray relative to the pixel of the initial ray. This change defines the pixel corresponding to the warped ray, and we specify Eq. (\textcolor{cvprblue}{11}) from the main paper:
\begin{equation}
	\begin{array}{ccc}
		\vspace{+1mm}
		\mathbf{p}^{t_{i}} = \left(\mathbf{p}(x_{t_{i}}), ~\mathbf{p}(y_{t_{i}})\right), \\
		\vspace{+1mm}
		\mathbf{p}(x_{t_{i+1}}) = \mathbf{p}(x_{t_{i}}) + \Delta\mathbf{p}(x_{t_{i+1}}), \\
		\mathbf{p}(y_{t_{i+1}}) = \mathbf{p}(y_{t_{i}}) + \Delta\mathbf{p}(y_{t_{i+1}}).
	\end{array}
\end{equation}
Following our assumption, the change in the initial ray must necessarily be zero, so we proposed the \textit{output suppression loss} to ensure it.

\section{Motion Blur in Real-World}
In real-world applications in 3D reconstruction, obtaining sharp images necessitates a small aperture size to ensure a substantial depth of field. This small aperture size inherently requires longer exposure times due to the diminished light intake, contradicting the assumption of very short exposure times. Longer exposure times inevitably lead to more intricate blur such as non-uniform blur as shown in \cref{fig:kernel}, which are not adequately represented by simple modelings such as linear motion assumptions.

 Therefore, using neural-ODEs to model camera motion  is particularly advantageous as they can accurately capture both linear and non-linear paths. The neural-ODEs are capable of representing a continuum of functions, thus effectively capturing the variations in camera motion regardless of their complexity or the amount of motion. Therefore, our approach is not only theoretically sound but also highly applicable in practical scenarios where the limitations of linear motion assumptions may lead to suboptimals.

 \begin{figure}[t]
 	\centering
 	\includegraphics[width=\linewidth]{figure1.pdf}
 	\caption{Blurry images caused by nonlinear camera path and kernels predicted by BAD-NeRF~\cite{wang2023bad} and our method.}
 	\label{fig:kernel}
 \end{figure}
 
 \section{Justification for Continuous Camera Motion}
 The impact of camera movements on image quality is profoundly influenced by the dynamic camera motion, including non-linear trajectories. Therefore, capturing the exact position and orientation of the camera is crucial, which is hard without considering the continuous nature of the motion~\cite{nayar2004motion}. While BAD-NeRF~\cite{wang2023bad} uses linear-spline interpolation for camera path estimation, our method surpasses BAD-NeRF, as detailed in the main paper. Spline models are useful for predictable movements, but they lack the flexibility to accurately model the intricate dynamics of camera motion that frequently occurs in real-world. They are constrained to fixed intervals and predefined degrees of freedom, which can oversimplify the motion path. With neural-ODEs, we consider sequences of continuous camera motion that were previously unaccounted for. This approach is advantageous as they can accurately capture both linear and non-linear paths. The neural-ODEs are capable of representing a continuum of functions, thus effectively capturing the variations in camera motion regardless of their motion complexity. As shown in \cref{fig:kernel}, while the warped rays of kernel of BAD-NeRF are linear, SMURF shows a non-linear camera motion path more close to actual motion blur. Therefore, our approach is not only theoretically sound but also highly applicable in practical scenarios where the limitations of linear motion assumptions may lead to suboptimals.
 
 While neural-ODEs may appear to be mathematically complex, they simply utilize neural networks to solve numerical differential equations, effectively combine traditional calculus with the learning capabilities of modern computing. They not only streamline the modeling of dynamic systems, but it is also straightforward to implement, making it a low-cost solution. Furthermore, it is important to clarify that our primary goal is to model continuous functions. The fact that the deblurring kernel is time-discrete does not contradict this objective. Ours is derived from a model that continuously defines the motion dynamics. We will revise this section to ensure clarity. Moreover, in real-world dataset of Deblur-NeRF~\cite{ma2022deblurnerf}, there is no ground truth for the actual camera path, and it is also impractical to obtain such ground truth in real scenarios, making it impossible to quantify the approximation error of the camera path.

\section{Number of Warped Rays}

We conduct extensive experiments to analyze the performance of the proposed CMBK based on the number of warped rays, $\mathcal{N}$. As shown in~\cref{tab:results}, larger $\mathcal{N}$ requires the more pixels to be rendered, resulting in an almost linear increase in training time. Moreover,~\cref{fig:num_warp} shows the performance according to the number of warped rays. Across all datasets, an increase in the number of warped rays tends to improve the PSNR and SSIM metrics. LPIPS noticeably decreases with more rays, interpreting that a higher number of warped rays ensures better perceptual quality. The performance for individual scenes in the synthetic dataset is shown in~\cref{tab:synthetic}, showing that LPIPS decreases with larger value of $\mathcal{N}$, and overall performance peaks when $\mathcal{N}$ is 8 or 9 except for the ``\textsc{Cozyroom}'' scene, . Analysis for the ``\textsc{Cozyroom}'' scene is conducted in~\cref{sec:analysis}. As indicated in~\cref{tab:synthetic_individual}, for the real-world dataset, a larger $\mathcal{N}$ generally guarantees higher performance across most scenes. However, there are scenes where performance drops when $\mathcal{N}$ exceeds 9, suggesting that the optimal $\mathcal{N}$ might be smaller than 9. Even with $\mathcal{N}$ set to 5, which is the same condition to DP-NeRF~\cite{lee2023dp} and Deblur-NeRF~\cite{ma2022deblurnerf}, SMURF outperforms them across all the metrics. Furthermore, SMURF achieves higher performance with fewer warped rays than PDRF-10~\cite{peng2023pdrf}, which set $\mathcal{N}$ at 10, validating the effectiveness of our proposed ideas.

\begin{table*}[!t] 
	\begin{center}
		\caption{Performance and training time of SMURF according to the number of warped rays. The \colorbox{best!25}{red}, \colorbox{second!25}{orange}, and \colorbox{third!25}{yellow} cells respectively indicate the highest, second-highest, and third-highest value.}
		\resizebox{0.8\linewidth}{!}{
		\centering
		\setlength{\tabcolsep}{4pt}
		\scriptsize
		\begin{tabular}{l|c|c|c|c|c|c|c|c}
			\toprule 
			
			\multirow{2}{*}{Methods~} 		& \multirow{2}{*}{~$\mathcal{N}$~}	   	& \multicolumn{3}{c|}{Synthetic Scene Dataset}  	   & \multicolumn{3}{c|}{Real-World Scene Dataset}  & \multirow{2}{*}{~Training Time (h)}\\ \cmidrule{3-8}
			& &~PSNR($\uparrow$)~    &~SSIM($\uparrow$)~    &~LPIPS($\downarrow$)~ &~PSNR($\uparrow$)~    &~SSIM($\uparrow$)~    &~LPIPS($\downarrow$)~     	& \\ \midrule \midrule
			SMURF	& 4	& 29.52	& 0.8829	& 0.1014	& 25.81	& 0.7710	& 0.1388 & 1.16 \\
			SMURF	& 5	& \cellcolor{third!25}30.30	& \cellcolor{third!25}0.9013	& 0.0926	& 25.91	& 0.7811	& 0.1253 & 1.27 \\
			SMURF	& 6	& 29.85	& 0.8929	& 0.0851	& 25.98	& 0.7822	& 0.1155 & 1.43\\
			SMURF	& 7	& 30.23	& 0.8964	& \cellcolor{third!25}0.0751	& \cellcolor{second!25}26.40	& \cellcolor{second!25}0.7944	& \cellcolor{third!25}0.1052 & 1.56\\
			SMURF	& 8	& \cellcolor{best!25}30.98	& \cellcolor{best!25}0.9147	& \cellcolor{second!25}0.0609	& \cellcolor{best!25}26.52	& \cellcolor{best!25}0.7986	& \cellcolor{best!25}0.1013 & 1.72\\
			SMURF	& 9	& \cellcolor{second!25}30.41	& \cellcolor{second!25}0.9086	& \cellcolor{best!25}0.0575	& \cellcolor{third!25}26.24	& \cellcolor{third!25}0.7922	& \cellcolor{second!25}0.1021 & 1.88 \\ \midrule
		\end{tabular}
	}
	\end{center}
	\label{tab:results}
\end{table*}

\begin{table*}[!t]
	\begin{center}
		\caption{Per-scene quantitative performance of SMURF, according to the number of warped rays.}
		\resizebox{\linewidth}{!}{
		\centering
		\setlength{\tabcolsep}{4pt}
		\scriptsize
		\begin{tabular}{l|c|c|c|c|c|c|c|c|c|c|c|c|c|c|c|c}
			\toprule 
			
			\multirow{2}{*}{Synthetic}  &\multirow{2}{*}{$\mathcal{N}$}			   & \multicolumn{3}{c|}{\textsc{Factory}}  	   & \multicolumn{3}{c|}{\textsc{CozyRoom}}  	   & \multicolumn{3}{c|}{\textsc{Pool}}  				& \multicolumn{3}{c|}{\textsc{Tanabata}} 		 & \multicolumn{3}{c}{\textsc{Trolley}}  \\ \cmidrule{3-17}
			&&PSNR     &SSIM     &LPIPS  &PSNR     &SSIM     &LPIPS 		&PSNR     &SSIM     &LPIPS 		&PSNR     &SSIM       &LPIPS 	&PSNR     &SSIM       &LPIPS   	\\ \midrule \midrule
			SMURF        &    4                 				 & 25.13	& 0.7697	& 0.2127	& \cellcolor{third!25}32.46	& \cellcolor{second!25}0.9294	& 0.0407	& \cellcolor{best!25}33.04	& \cellcolor{best!25}0.8993	& 0.0825	& 28.38	& 0.9059	& 0.0825	& 28.57	& 0.9101	& 0.0890 \\
			SMURF        &     5               				& 27.33	& 0.8381	& 0.2075	& \cellcolor{best!25}32.72	& \cellcolor{best!25}0.9315	& \cellcolor{best!25}0.0375	& 32.47	& 0.8904	& 0.0797	& \cellcolor{third!25}29.34	& \cellcolor{third!25}0.9222	& 0.0631	& \cellcolor{third!25}29.65	& \cellcolor{third!25}0.9241	& 0.0755 \\
			SMURF		&		6							& \cellcolor{third!25}26.74	& \cellcolor{third!25}0.8159	& 0.1897	& 31.74	& 0.9246	& 0.0381	& \cellcolor{third!25}32.56	& \cellcolor{third!25}0.8922	& \cellcolor{third!25}0.0778	& 29.22	& 0.9179	& 0.0604	& 28.99	& 0.9139	& 0.0599 \\ 
			SMURF        &       7          				& 26.15	& 0.8010	& \cellcolor{third!25}0.1679	& 32.12	& 0.9269	& \cellcolor{second!25}0.0378	& \cellcolor{second!25}32.59	& \cellcolor{second!25}0.8926	& \cellcolor{second!25}0.0773	& \cellcolor{second!25}29.69	& \cellcolor{second!25}0.9269	& \cellcolor{third!25}0.0490	& \cellcolor{best!25}30.58	& \cellcolor{best!25}0.9348	& \cellcolor{third!25}0.0438   \\
			SMURF         &      8          				& \cellcolor{second!25}29.87	& \cellcolor{second!25}0.8958	& \cellcolor{second!25}0.1057	& \cellcolor{second!25}32.48	& \cellcolor{third!25}0.9285	& \cellcolor{third!25}0.0379	& 32.34	& 0.8884	& 0.0779	& \cellcolor{best!25}29.91	& \cellcolor{best!25}0.9300	& \cellcolor{best!25}0.0436	& \cellcolor{second!25}30.30	& \cellcolor{second!25}0.9307	& \cellcolor{best!25}0.0397    \\
			SMURF          &      9         				& \cellcolor{best!25}30.52	& \cellcolor{best!25}0.9065	& \cellcolor{best!25}0.0807	& 31.43	& 0.9198	& 0.0428	& 32.10	& 0.8849	& \cellcolor{best!25}0.0771	& 28.93	& 0.9184	& \cellcolor{second!25}0.0448	& 29.05	& 0.9136	& \cellcolor{second!25}0.0423    \\ 
			
			\midrule \midrule
			
			\multirow{2}{*}{Real}  &\multirow{2}{*}{$\mathcal{N}$}			   & \multicolumn{3}{c|}{\textsc{Ball}}  	   & \multicolumn{3}{c|}{\textsc{Basket}}  	   & \multicolumn{3}{c|}{\textsc{Buick}}  				& \multicolumn{3}{c|}{\textsc{Coffee}} 		 & \multicolumn{3}{c}{\textsc{Decoration}}  \\ \cmidrule{3-17}
			&&PSNR     &SSIM     &LPIPS  &PSNR     &SSIM     &LPIPS 		&PSNR     &SSIM     &LPIPS 		&PSNR     &SSIM       &LPIPS 	&PSNR     &SSIM       &LPIPS   	\\ \midrule \midrule
			SMURF	& 4	& 26.47	& 0.7424	& 0.1754	& 28.30	& 0.8653	& 0.0847	& 26.57	& 0.8270	& 0.1066	& 30.66	& 0.8676	& 0.1228	& \cellcolor{third!25}24.59	& \cellcolor{third!25}0.7972	& 0.1471 \\
			SMURF	& 5	& 26.63	& 0.7528	& 0.1549	& 27.96	& 0.8648	& 0.0741	& 26.03	& 0.8254	& 0.0947	& \cellcolor{third!25}30.93	& \cellcolor{third!25}0.8734	& 0.1172	& 24.22	& 0.7799	& 0.1497 \\
			SMURF	& 6	& \cellcolor{third!25}27.31	& 0.7678	& 0.1434	& 27.19	& 0.8463	& 0.0773	& 26.75	& 0.8315	& 0.0905	& 30.76	& 0.8731	& 0.1004	& 24.16	& 0.7744	& 0.1465 \\
			SMURF	& 7	& \cellcolor{best!25}27.68	& \cellcolor{best!25}0.7821	& \cellcolor{third!25}0.1325	& \cellcolor{best!25}29.24	& \cellcolor{best!25}0.8862	& \cellcolor{best!25}0.0617	& \cellcolor{second!25}27.05	& \cellcolor{second!25}0.8395	& \cellcolor{third!25}0.0867	& 30.67	& 0.8649	& \cellcolor{third!25}0.0931	& \cellcolor{best!25}24.97	& \cellcolor{second!25}0.8092	& \cellcolor{second!25}0.1220 \\
			SMURF	& 8	& \cellcolor{second!25}27.50	& \cellcolor{second!25}0.7760	& \cellcolor{best!25}0.1298	& \cellcolor{second!25}28.95	& \cellcolor{second!25}0.8842	& \cellcolor{second!25}0.0619	& \cellcolor{best!25}27.10	& \cellcolor{best!25}0.8409	& \cellcolor{second!25}0.0839	& \cellcolor{second!25}31.33	& \cellcolor{best!25}0.8879	& \cellcolor{second!25}0.0874	& \cellcolor{second!25}24.90	& \cellcolor{best!25}0.8114	& \cellcolor{best!25}0.1190 \\
			SMURF	& 9	& 27.16	& \cellcolor{third!25}0.7698	& \cellcolor{second!25}0.1315	& \cellcolor{third!25}28.52	& \cellcolor{third!25}0.8766	& \cellcolor{third!25}0.0631	& \cellcolor{third!25}26.92	& \cellcolor{third!25}0.8366	& \cellcolor{best!25}0.0813	& \cellcolor{best!25}31.41	& \cellcolor{second!25}0.8802	& \cellcolor{best!25}0.0870	& 24.12	& 0.7753	& \cellcolor{third!25}0.1405   \\ \midrule \midrule
			
			\multirow{2}{*}{Real}  &\multirow{2}{*}{~$\mathcal{N}$~}			   & \multicolumn{3}{c|}{\textsc{Girl}}  	   & \multicolumn{3}{c|}{\textsc{Heron}}  	   & \multicolumn{3}{c|}{\textsc{Parterre}}  				& \multicolumn{3}{c|}{\textsc{Puppet}} 		 & \multicolumn{3}{c}{\textsc{Stair}}  \\ \cmidrule{3-17}
			&&PSNR     &SSIM     &LPIPS  &PSNR     &SSIM     &LPIPS 		&PSNR     &SSIM     &LPIPS 		&PSNR     &SSIM       &LPIPS 	&PSNR     &SSIM       &LPIPS   	\\ \midrule \midrule
			SMURF	& 4	& 24.66	& 0.8410	& 0.1084	& 23.36	& 0.7144	& 0.1863	& \cellcolor{second!25}25.43	& \cellcolor{third!25}0.7644	& 0.1611	& 24.63	& 0.7496	& 0.1277	& 23.38	& 0.5406	& 0.1687 \\
			SMURF	& 5	& 24.73	& 0.8354	& 0.1028	& 23.47	& 0.7244	& 0.1717	& \cellcolor{third!25}25.22	& 0.7640	& 0.1474	& 24.69	& 0.7514	& 0.1239	& 25.22	& \cellcolor{second!25}0.6391	& 0.1171 \\
			SMURF	& 6	& 25.10	& 0.8473	& 0.0940	& \cellcolor{third!25}23.60	& \cellcolor{second!25}0.7386	& 0.1533	& 24.99	& 0.7569	& 0.1402	& 24.51	& 0.7493	& 0.1145	& \cellcolor{third!25}25.38	& \cellcolor{third!25}0.6371	& 0.0956 \\
			SMURF	& 7	& \cellcolor{third!25}25.43	& \cellcolor{second!25}0.8570	& \cellcolor{third!25}0.0884	& \cellcolor{second!25}23.66	& \cellcolor{third!25}0.7352	& \cellcolor{third!25}0.1457	& \cellcolor{third!25}25.22	& \cellcolor{second!25}0.7744	& \cellcolor{third!25}0.1302	& \cellcolor{third!25}24.70	& \cellcolor{second!25}0.7587	& \cellcolor{second!25}0.1076	& \cellcolor{second!25}25.42	& 0.6370	& \cellcolor{third!25}0.0846 \\
			SMURF	& 8	& \cellcolor{best!25}25.66	& \cellcolor{best!25}0.8592	& \cellcolor{second!25}0.0829	& 23.59	& 0.7317	& \cellcolor{second!25}0.1381	& \cellcolor{best!25}25.47	& \cellcolor{best!25}0.7825	& \cellcolor{best!25}0.1207	& \cellcolor{best!25}25.19	& \cellcolor{best!25}0.7702	& \cellcolor{third!25}0.1077	& \cellcolor{best!25}25.48	& \cellcolor{best!25}0.6421	& \cellcolor{second!25}0.0822 \\
			SMURF	& 9	& \cellcolor{second!25}25.56	& \cellcolor{third!25}0.8567	& \cellcolor{best!25}0.0822	& \cellcolor{best!25}23.81	& \cellcolor{best!25}0.7828	& \cellcolor{best!25}0.1333	& 24.91	& 0.7583	& \cellcolor{second!25}0.1216	& \cellcolor{second!25}24.71	& \cellcolor{third!25}0.7554	& \cellcolor{best!25}0.1035	& 25.31	& 0.6302	& \cellcolor{best!25}0.0777  \\ \bottomrule
		\end{tabular}
	}
	\end{center}
	\label{tab:synthetic}
\end{table*}

\begin{figure*}[t]
	\centering
	\includegraphics[width=\linewidth]{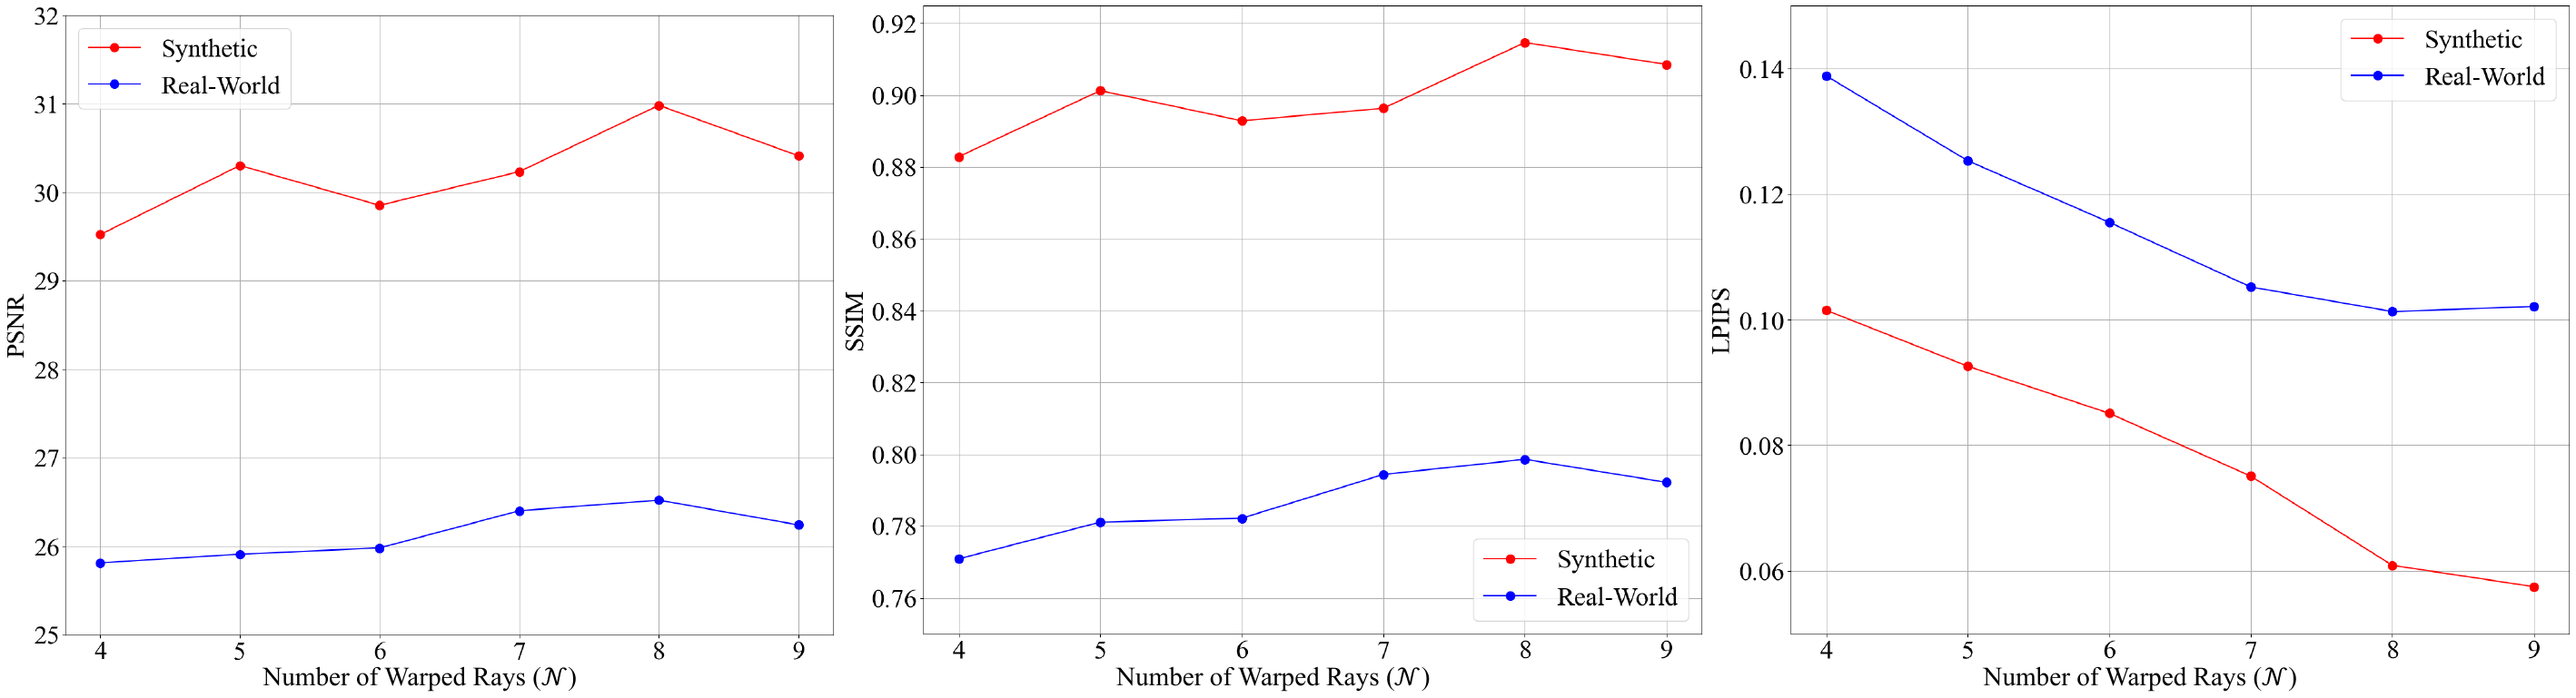}
	\caption{Variation in performance with the number of warped rays.}
	\label{fig:num_warp}
\end{figure*}

\clearpage

\twocolumn[{
	\renewcommand\twocolumn[1][]{#1}
	\begin{center}
		\centering
		\captionsetup{type=figure}
		\includegraphics[width=1\linewidth]{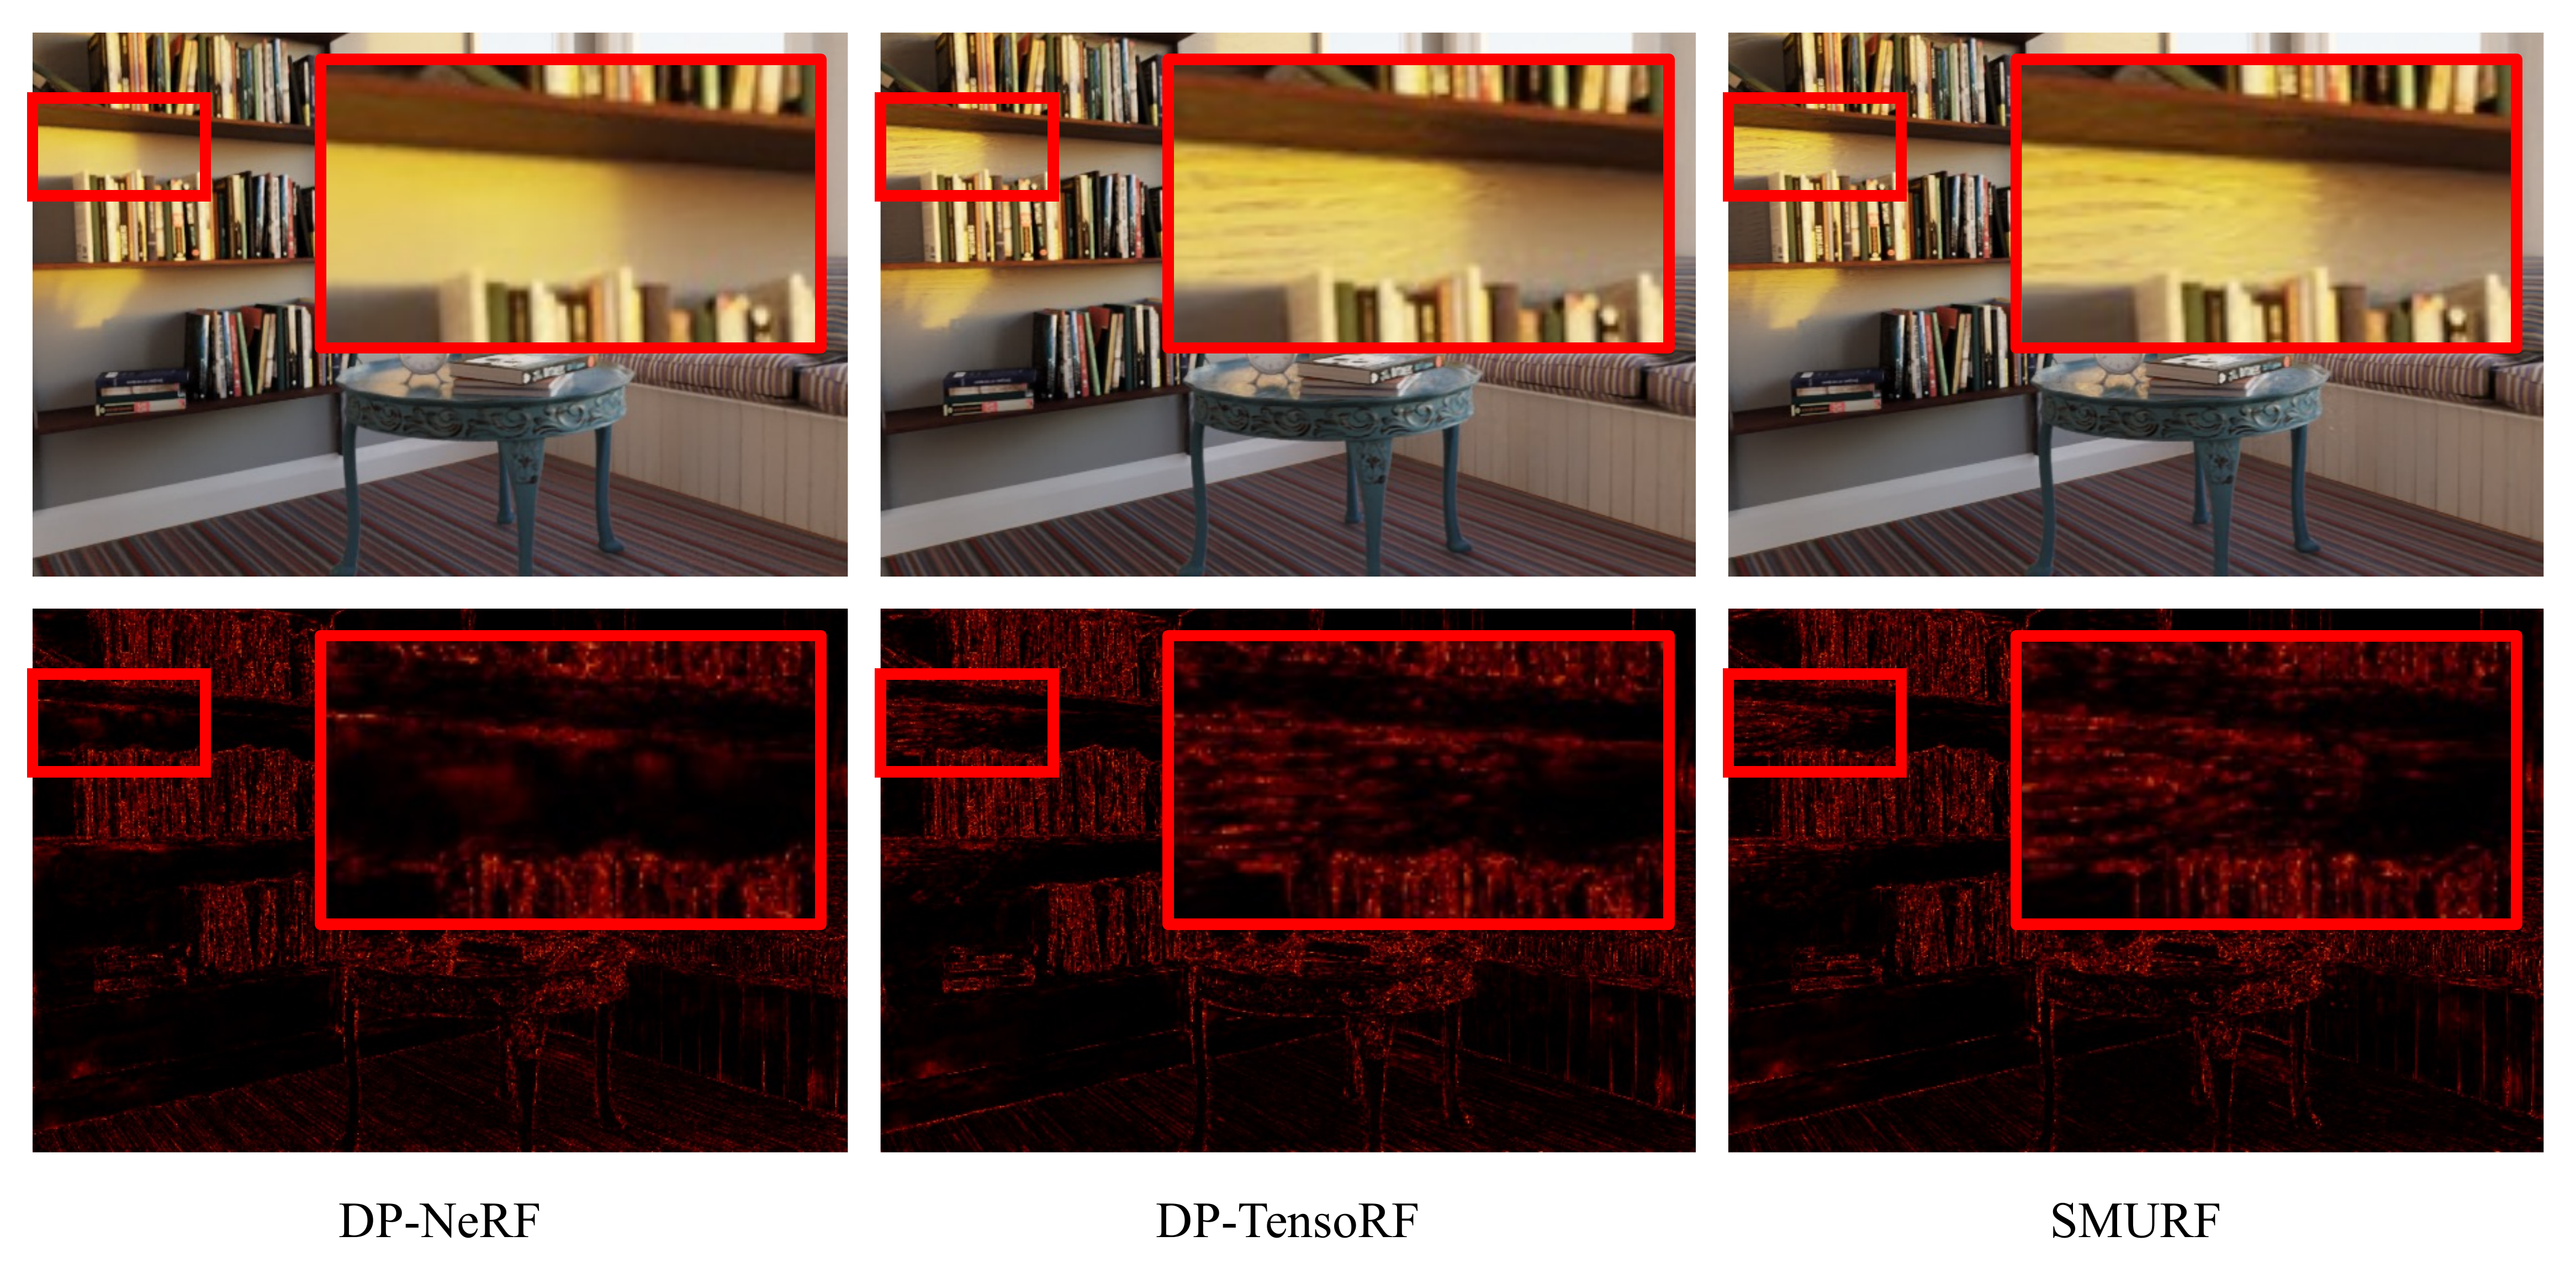}
		\caption{\textbf{Qualitative comparison of rendering results and error maps for the Cozyroom scene.} DP-TensoRF is a model that applies the kernel proposed by DP-NeRF~\cite{lee2023dp} to TensoRF~\cite{chen2022tensorf}.}
		\label{fig:cozyroom}
	\end{center}
}]

\section{Analysis for Low-PSNR Scenes} \label{sec:analysis}

In this section, we analyze individual scenes that showed slightly lower performance from the main paper. Notably, we visualize the error maps for the ``\textsc{Cozyroom}'' scene from the synthetic dataset for DP-NeRF~\cite{lee2023dp}, DP-TensoRF~\cite{lee2023dp,chen2022tensorf}, and SMURF in~\cref{fig:cozyroom}, where DP-TensoRF is a model that applies the blurring kernel proposed by DP-NeRF to TensoRF. The error map for DP-NeRF shows bright wall rendered cleanly without noise, whereas DP-TensoRF and SMURF exhibit noise on the wall. This indicates that the cause of noise is not the proposed CMBK but the inherent characteristics of the backbone model, TensoRF. As shown in~\cref{fig:render_synthetic}, aside from the noise on the wall, the rendering results of SMURF show slightly sharper image quality in other areas except the wall. Moreover, the ``\textsc{Coffee}'', ``\textsc{Parterre}'', and ``\textsc{Puppet}" scenes from real-world dataset, SMURF shows the best LPIPS score but somewhat lower PSNR. However, when comparing the rendering results in~\cref{fig:render_synthetic,fig:render_real_1}, it is observable that the results of SMURF are most similar to the reference images for these scenes.

\section{Limitations and Future Work}

By adopting TensoRF~\cite{chen2022tensorf}, a 3D tensor factorization-based method, as our backbone, we ensure high quantitative performance, superior perceptual quality, and faster training. However, with the advent of 3D Gaussian Splatting~\cite{kerbl20233d}, which allows for GPU-based rasterization instead of optimizing per ray, backbones that facilitate more faster training and rendering become available. Although our backbone may be slower compared to 3D Gaussian Splatting, applying the main idea of CMBK, \textit{continuous dynamics}, to a rasterization-based method is expected to result in faster training and rendering. Furthermore, by demonstrating the applicability of \textit{continuous dynamics} to the 3D scene deblurring, we anticipate the possibility of designing models that cover not only camera motion blur but also object motion blur, which is caused by the movement of objects within the scene.

\section{Per-Scene Quantitative Results}

To demonstrate the superiority of SMURF, we present the individual performance results for all synthetic and real-world scenes in~\cref{tab:synthetic_individual}. For synthetic scenes, except for ``\textsc{Cozyroom},'' all scenes show quantitatively high performance, with this scene also displaying no significant difference when compared to DP-NeRF. Additionally, for the real-world scenes, despite a few scenes exhibiting somewhat lower PSNR, they demonstrate better perceptual quality through superior LPIPS scores. For a fair comparison, we also include the performance of DP-TensoRF, which applies the state-of-the-art DP-NeRF~\cite{lee2023dp} to the explicit volumetric rendering method using the TensoRF~\cite{chen2022tensorf} backbone. Although DP-TensoRF benefits from reduced training time due to the use of the TensoRF backbone, it shows negligible performance differences when compared to DP-NeRF, and our SMURF outperforms both. Notably, DP-TensoRF generally exhibits lower PSNR and SSIM scores than DP-NeRF on real-world scenes. This indicates that the performance of our SMURF is not significantly dependent on the TensoRF backbone.

\begin{table*}[!t]
	\begin{center}
		\resizebox{\linewidth}{!}{
			\centering
			\setlength{\tabcolsep}{4pt}
			\scriptsize
			\begin{tabular}{l||c|c|c|c|c|c|c|c|c|c|c|c|c|c|c}
				\toprule 
				
				\multirow{2}{*}{Synthetic} 			   & \multicolumn{3}{c|}{\textsc{Factory}}  	   & \multicolumn{3}{c|}{\textsc{CozyRoom}}  	   & \multicolumn{3}{c|}{\textsc{Pool}}  				& \multicolumn{3}{c|}{\textsc{Tanabata}} 		 & \multicolumn{3}{c}{\textsc{Trolley}}  \\ \cmidrule{2-16}
				&PSNR     &SSIM     &LPIPS  &PSNR     &SSIM     &LPIPS 		&PSNR     &SSIM     &LPIPS 		&PSNR     &SSIM       &LPIPS 	&PSNR     &SSIM       &LPIPS   	\\ \midrule \midrule
				Naive NeRF                            				 & 19.32    & 0.4563   & 0.5304 		& 25.66       & 0.7941      & 0.2288      & 30.45    & 0.8354      & 0.1932    		& 22.22    & 0.6807      & 0.3653    		& 21.25    & 0.6370     & 0.3633    \\
				MPR+NeRF                            				& 21.70    & 0.6153   & 0.3094 			& 27.88       & 0.8502      & 0.1153      & 30.64    & 0.8385      & 0.1641    		& 22.71    & 0.7199      & 0.2509    		& 22.64    & 0.7141     & 0.2344    \\ 
				PVD+NeRF											& 20.33		& 0.5386 & 0.3667			& 27.74 	& 0.8296		& 0.1451		& 27.56	& 0.7626		& 0.2148		& 23.44	& 0.7293		& 0.2542			&23.81	& 0.7351	& 0.2567 \\ \midrule		
				Deblur-NeRF                         				& 25.60    & 0.7750   & 0.2687 		 & 32.08       & 0.9261      & 0.0477        & 31.61     & 0.8682      & 0.1246    		& 27.11     & 0.8640      & 0.1228    		 & 27.45    & 0.8632     & 0.1363    \\
				%				PDRF-10                         					   & \cellcolor{second!35}26.56    & 0.8102   & - 		 		  & 31.90       & 0.9321      & -        			& 31.29     & 0.8657      & -    				& \cellcolor{second!35}28.21     & \cellcolor{second!35}0.8952      & -    		 		 & \cellcolor{second!35}28.48    & \cellcolor{second!35}0.8956     & - 		    \\
				PDRF-10*                         					   & 25.87    & \cellcolor{second!35}0.8316   & \cellcolor{second!35}0.1915 		 		  & 31.13       &  0.9225     & 0.0439        			& 31.00     & 0.8583      & 0.1408    				& 28.01     & 0.8931      & 0.1004    		 		 & 28.29    & 0.8921     & \cellcolor{second!35}0.0931 		    \\
				BAD-NeRF*                         				& 24.43    & 0.7274   & 0.2134 		 & 29.77       & 0.8864      & 0.0616        & 31.51     & 0.8620      & \cellcolor{second!35}0.0802    		& 25.32     & 0.8081      & 0.1077    		 & 25.58    & 0.8049     & 0.1008    \\
				DP-NeRF                        						  & \cellcolor{second!35}25.91    & 0.7787   & 0.2494 		& \cellcolor{best!25}32.65   	 & \cellcolor{best!25}0.9317      & \cellcolor{best!25}0.0355    		& 31.96    & 0.8768      & 0.0908    	& 27.61    & 0.8748      & 0.1033    		& 28.03    & 0.8752      & 0.1129   \\ \midrule 
				DP-TensoRF                         				& 25.54    & 0.7798   & 0.2250 		 & 32.13       & 0.9252      & 0.0397        & \cellcolor{second!35}32.14     & \cellcolor{second!35}0.8826      & 0.0877    		& \cellcolor{second!35}28.22     & \cellcolor{second!35}0.9007      & \cellcolor{second!35}0.0917    		 & \cellcolor{second!35}28.59    & \cellcolor{second!35}0.9075     & 0.0963    \\ \midrule \midrule
				\textbf{SMURF}                         						   & \cellcolor{best!25}29.87    & \cellcolor{best!25}0.8958   & \cellcolor{best!25}0.1057 		 & \cellcolor{second!35}32.48   		& \cellcolor{second!35}0.9285      & \cellcolor{second!35}0.0379    	& \cellcolor{best!25}32.34    & \cellcolor{best!25}0.8884      & \cellcolor{best!25}0.0779   	 & \cellcolor{best!25}29.91    & \cellcolor{best!25}0.9300      & \cellcolor{best!25}0.0436    		& \cellcolor{best!25}30.30    & \cellcolor{best!25}0.9307      & \cellcolor{best!25}0.0397   \\ 
				
				\midrule \midrule
				\multirow{2}{*}{Real-World} 			   & \multicolumn{3}{c|}{\textsc{Ball}}  	   & \multicolumn{3}{c|}{\textsc{Basket}}  	   & \multicolumn{3}{c|}{\textsc{Buick}}  				& \multicolumn{3}{c|}{\textsc{Coffee}} 		 & \multicolumn{3}{c}{\textsc{Decoration}}  \\ \cmidrule{2-16}
				&PSNR     &SSIM     &LPIPS  &PSNR     &SSIM     &LPIPS 		&PSNR     &SSIM     &LPIPS 		&PSNR     &SSIM       &LPIPS 	&PSNR     &SSIM       &LPIPS   	\\ \midrule \midrule
				Naive NeRF                            				 & 24.08    & 0.6237   & 0.3992 		& 23.72       & 0.7086      & 0.3223      & 21.59    & 0.6325      & 0.3502    		& 26.48    & 0.8064      & 0.2896    		& 22.39    & 0.6609     & 0.3633    \\ \midrule
				Deblur-NeRF                         				& 27.36    & 0.7656   & 0.2230 		 & 27.67       & 0.8449      & 0.1481        & 24.77     & 0.7700      & 0.1752    		& 30.93     & 0.8981      & 0.1244    		 & 24.19    & 0.7707     & 0.1862    \\
				PDRF-10*                            				 & \cellcolor{second!35}27.37    & \cellcolor{second!35}0.7642   & 0.2093 		& \cellcolor{second!35}28.36       & \cellcolor{second!35}0.8736      & \cellcolor{second!35}0.1179      & 25.73    & 0.7916      & 0.1582    		& \cellcolor{best!25}31.79    & \cellcolor{second!25}0.9002      & 0.1133    		& 23.55   & 0.7508     & 0.2145    \\ 
				BAD-NeRF*                            				 & 21.33 & 0.5096 & 0.4692 & 26.44 & 0.8080 & 0.1325 & 21.63 & 0.6429 & 0.2593 & 28.98 & 0.8369 & 0.1956 & 22.13 & 0.6316 & 0.2894    \\ 
				DP-NeRF                        						  & 27.20    & 0.7652   & \cellcolor{second!35}0.2088 		& 27.74   	 & 0.8455      & 0.1294    		& \cellcolor{second!35}25.70    & \cellcolor{second!35}0.7922      & \cellcolor{second!35}0.1405    	& 31.19    & \cellcolor{best!25}0.9049      & \cellcolor{second!35}0.1002    		& \cellcolor{second!35}24.31    & \cellcolor{second!35}0.7811     & \cellcolor{second!35}0.1639   \\ \midrule 
				DP-TensoRF                         				& 25.85    & 0.7164   & 0.2106 		 & 27.04       & 0.8434      & \cellcolor{second!35}0.1099        & 25.02     & 0.7981      & 0.1603    		& 29.67     & 0.8424      & 0.1323    		 & 22.78    & 0.7362     & 0.1801    \\ \midrule \midrule
				\textbf{SMURF}                         						   & \cellcolor{best!25}27.50    & \cellcolor{best!25}0.7760   & \cellcolor{best!25}0.1298 		 & \cellcolor{best!25}28.95   		& \cellcolor{best!25}0.8842      & \cellcolor{best!25}0.0619    	& \cellcolor{best!25}27.10    & \cellcolor{best!25}0.8409      & \cellcolor{best!25}0.0839   	 & \cellcolor{second!35}31.33    & 0.8879      & \cellcolor{best!25}0.0874    		& \cellcolor{best!25}24.90    & \cellcolor{best!25}0.8114      & \cellcolor{best!25}0.1190   \\ \midrule \midrule
				
				\multirow{2}{*}{Real-World} 			   & \multicolumn{3}{c|}{\textsc{Girl}}  	   & \multicolumn{3}{c|}{\textsc{Heron}}  	   & \multicolumn{3}{c|}{\textsc{Parterre}}  				& \multicolumn{3}{c|}{\textsc{Puppet}} 		 & \multicolumn{3}{c}{\textsc{Stair}}  \\ \cmidrule{2-16}
				&PSNR     &SSIM     &LPIPS  &PSNR     &SSIM     &LPIPS 		&PSNR     &SSIM     &LPIPS 		&PSNR     &SSIM       &LPIPS 	&PSNR     &SSIM       &LPIPS   	\\ \midrule \midrule
				Naive NeRF                            				 & 20.07    & 0.7075   & 0.3196 		& 20.50       & 0.5217      & 0.4129      & 23.14    & 0.6201      & 0.4046    		& 22.09    & 0.6093      & 0.3389    		& 22.87    & 0.4561     & 0.4868    \\ \midrule
				Deblur-NeRF                         				& 22.27    & 0.7976   & 0.1687 		 & 22.63       & 0.6874      & 0.2099        & \cellcolor{second!35}25.82     & 0.7597      & 0.2161    		& \cellcolor{second!35}25.24     & 0.7510      & 0.1577    		 & 25.39    & 0.6296     & 0.2102    \\
				PDRF-10*                            				 & \cellcolor{second!35}24.12    & \cellcolor{second!35}0.8328   & 0.1679 		& 22.53       & 0.6880      & 0.2358      & 25.36    & 0.7601      & 0.2263    		& 25.02    & 0.7496     & 0.1532    		& 25.20    & 0.6235     & 0.2288    \\ 
				BAD-NeRF*                            				 & 18.10 & 0.5652 & 0.3933 & 22.18 & 0.6479 & 0.2226 & 23.44 & 0.6243 & 0.3151 & 22.48 & 0.6249 & 0.2762 & 21.52 & 0.4237 & 0.3341    \\ 
				DP-NeRF                        						  & 23.33    & 0.8139   & \cellcolor{second!35}0.1498 		& \cellcolor{second!35}22.88   	 & \cellcolor{second!35}0.6930      & \cellcolor{second!35}0.1914    		& \cellcolor{best!25}25.86    & 0.7665      & 0.1900    	& \cellcolor{best!25}25.25    & \cellcolor{second!35}0.7536      & 0.1505    		& \cellcolor{best!25}25.59    & \cellcolor{second!25}0.6349      & 0.1772   \\ \midrule
				DP-TensoRF                         				& 21.32    & 0.7775   & 0.1614 		 & 22.62       & 0.6861      & 0.2039        & 25.37     & \cellcolor{second!35}0.7708      & \cellcolor{second!35}0.1761    		& 24.29     & 0.7376      & \cellcolor{second!35}0.1495    		 & 23.52    & 0.6022     & \cellcolor{second!35}0.1752    \\ \midrule \midrule
				\textbf{SMURF}                         						   &\cellcolor{best!25}25.66    & \cellcolor{best!25}0.8592   & \cellcolor{best!25}0.0829 		 & \cellcolor{best!25}23.59   		& \cellcolor{best!25}0.7317      & \cellcolor{best!25}0.1381    	& 25.47    & \cellcolor{best!25}0.7825     & \cellcolor{best!25}0.1207   	 & 25.19    & \cellcolor{best!25}0.7702      & \cellcolor{best!25}0.1077    			& \cellcolor{second!35}25.48    & \cellcolor{best!25}0.6421      & \cellcolor{best!25}0.0822  \\ \bottomrule
			\end{tabular}
		}
	\end{center}
	\caption{\textbf{Comparison of performance for individual scenes.} SMURF exhibits higher performance across all synthetic scenes, with the exception of ``\textsc{CozyRoom},'' where it shows slightly lower performance relative to others. For real-world scenes, while SMURF shows slightly lower PSNR and SSIM in some scenes, it shows significantly better LPIPS across all scenes compared to previous methods.}
	\label{tab:synthetic_individual}
\end{table*}

\section{Additional Rendering Results} % Cozyroom, Coffee, Parterre, Puppet

Additional rendering results are shown in~\cref{fig:render_synthetic} and~\cref{fig:render_real_1}, demonstrating that our SMURF offers the best perceptual quality when compared to the reference images. Please refer to the \textit{supplementary videos} for comparisons of rendered videos.

\begin{figure*}[t]
	\centering
	\includegraphics[width=\linewidth]{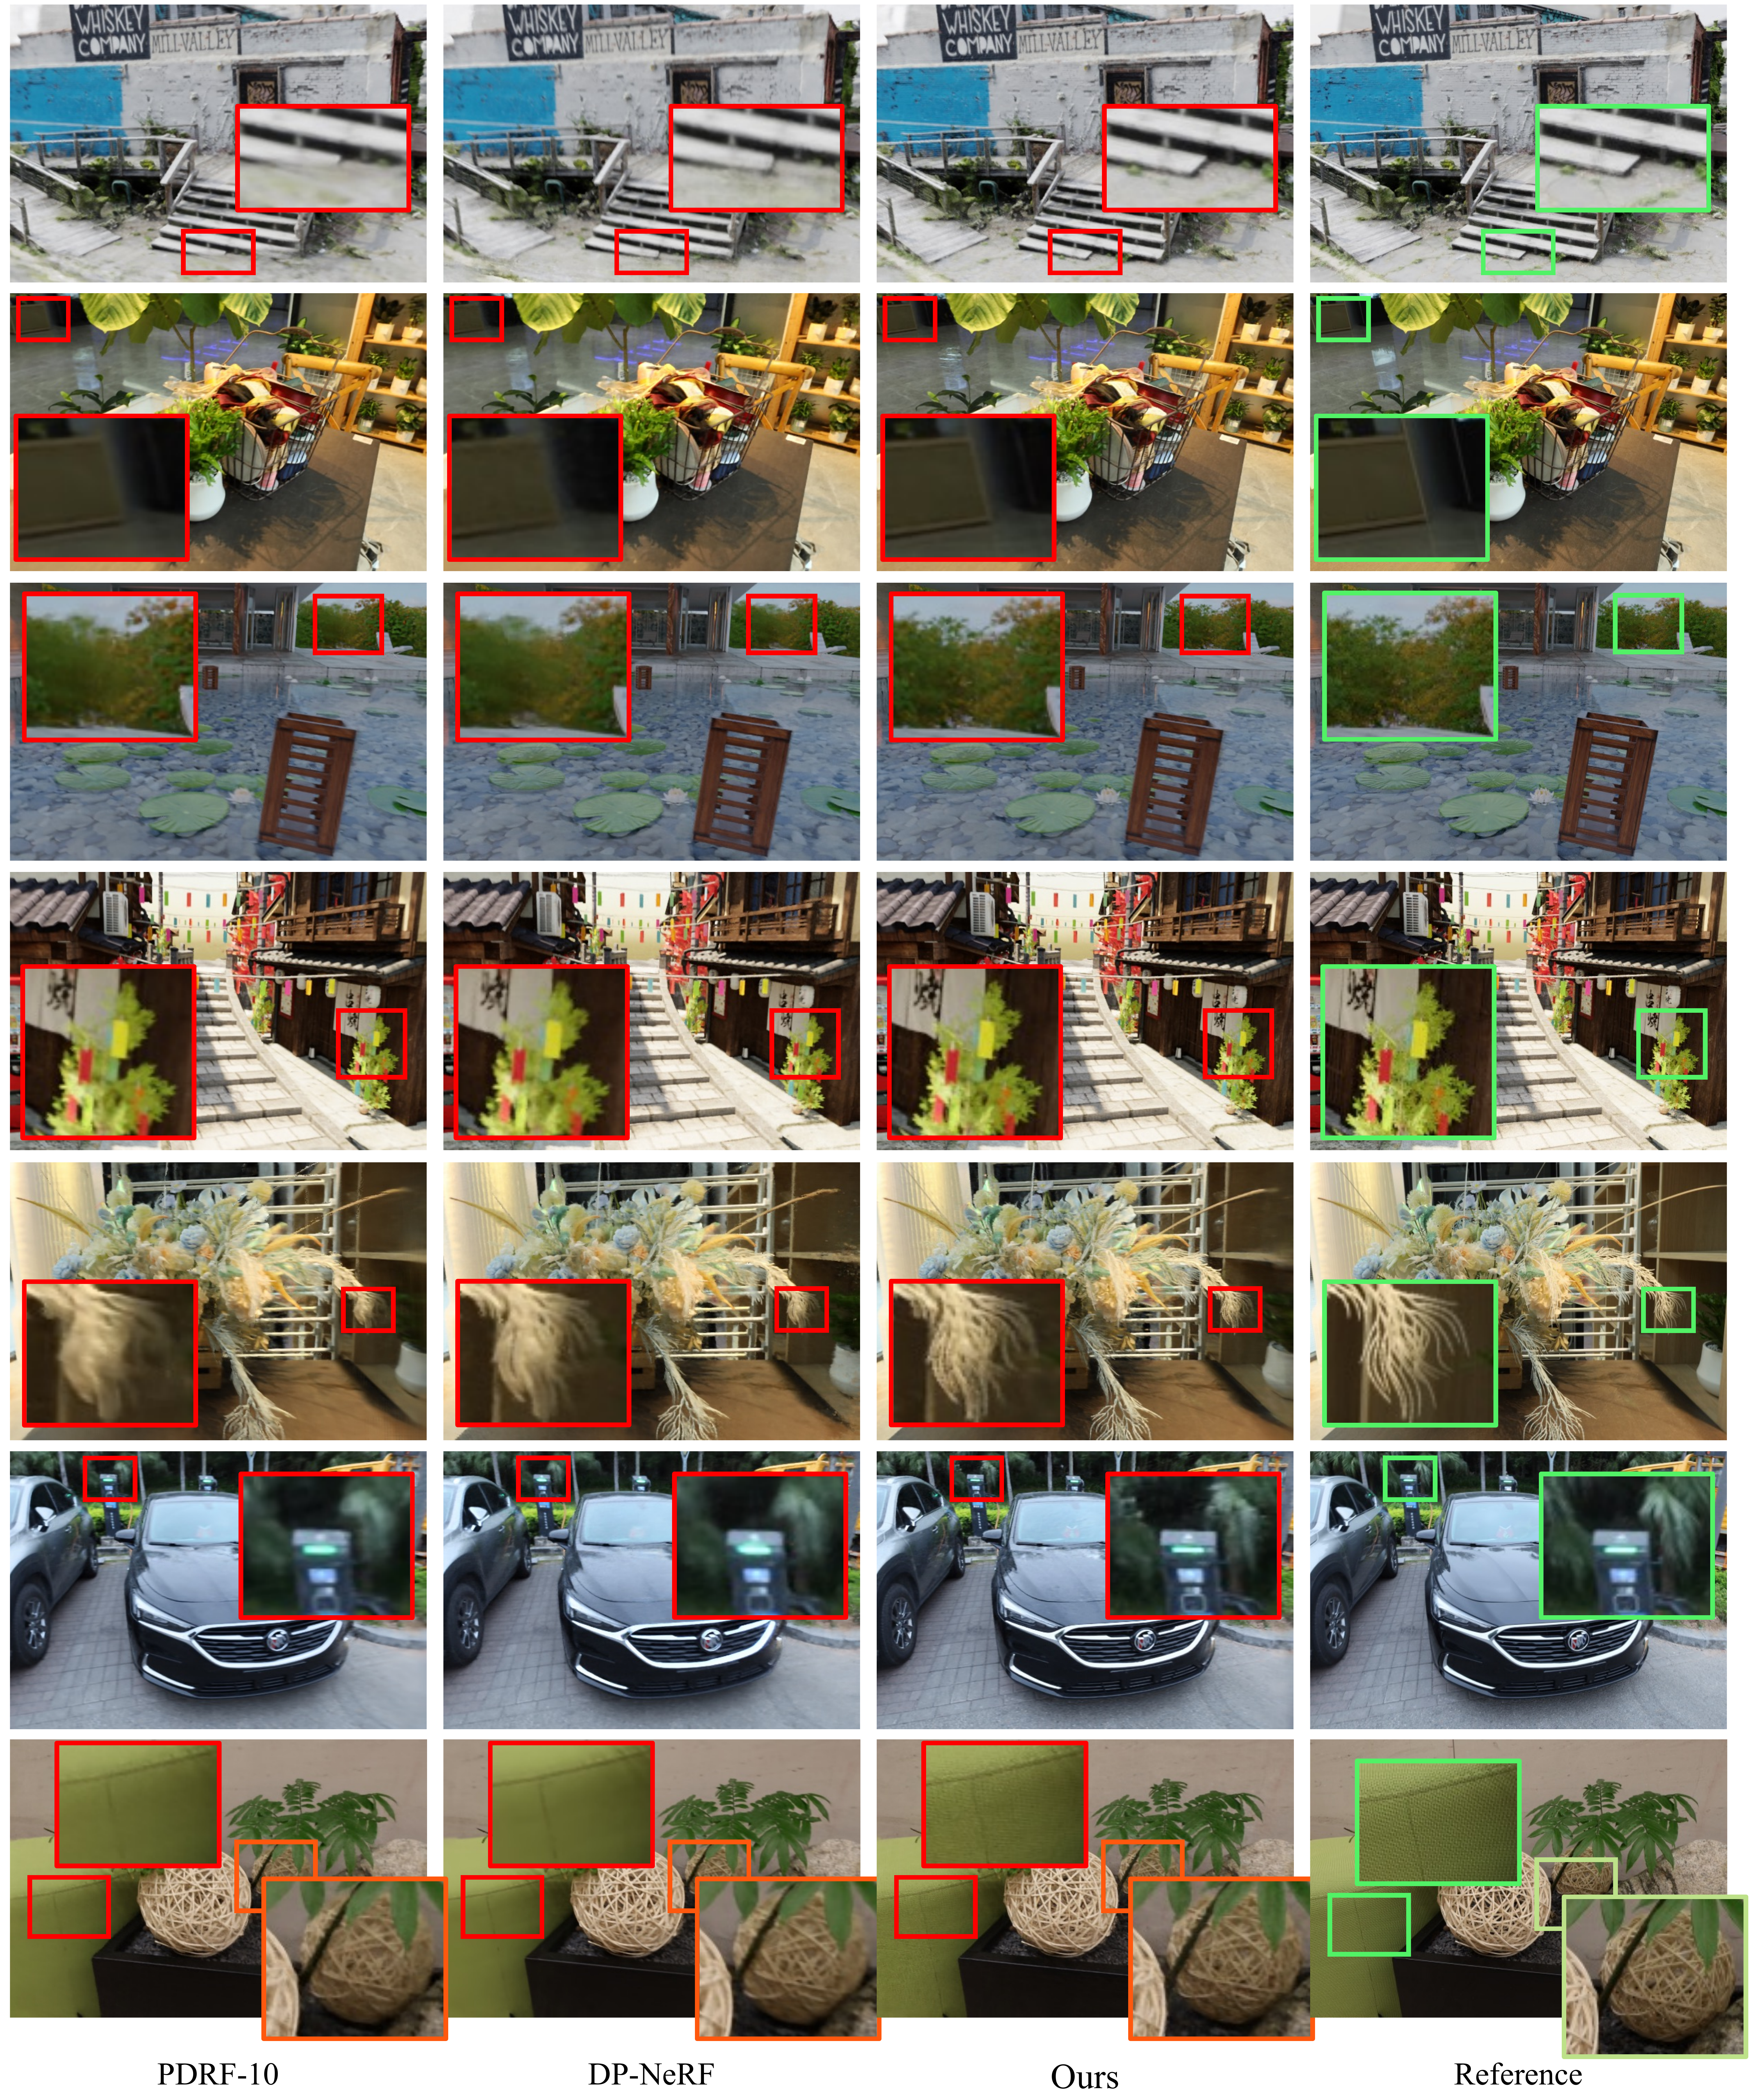}
	\caption{Qualitative comparison for individual scenes.}
	\label{fig:render_synthetic}
\end{figure*}
% Synthetic dataset의 개별 scene에 따른 정성적 비교

\begin{figure*}[t]
	\centering
	\includegraphics[width=\linewidth]{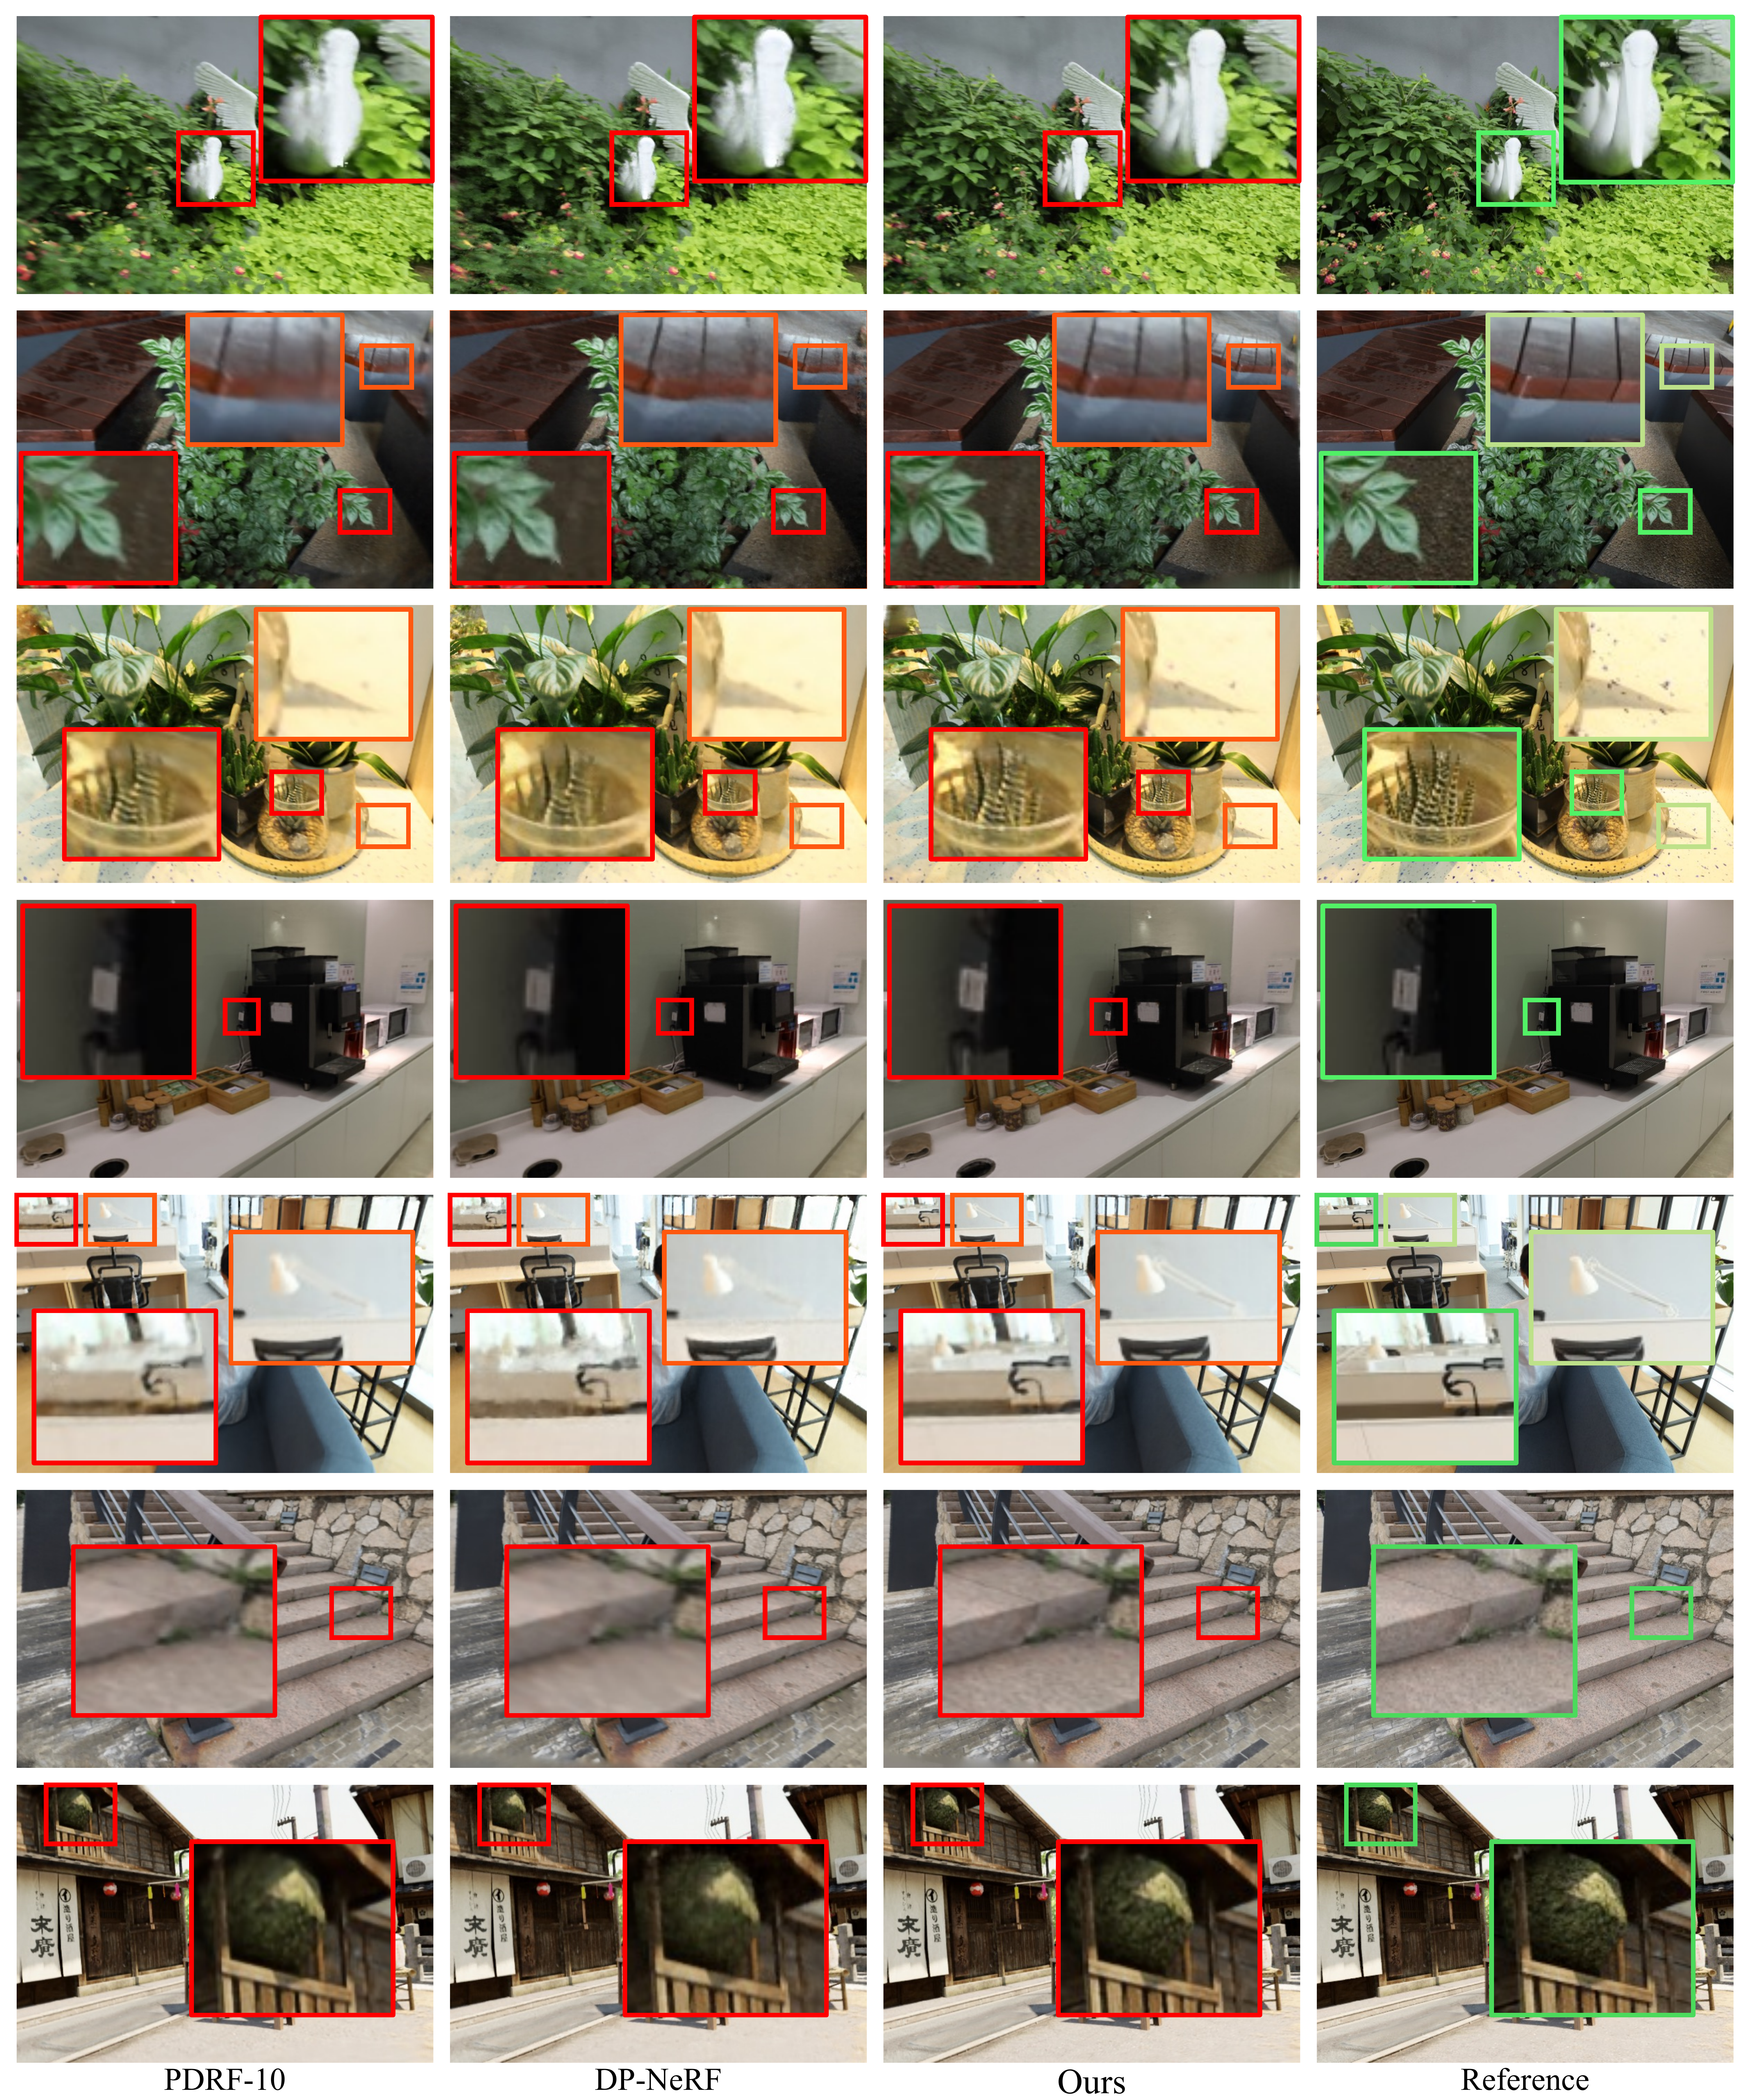}
	\caption{Qualitative comparison for individual scenes.}
	\label{fig:render_real_1}
\end{figure*}
