# Supplementary material for: SMURF: Continuous Dynamics for Motion-Deblurring Radiance Fields
Source: arXiv:2403.07547 source file (2025-05-15)

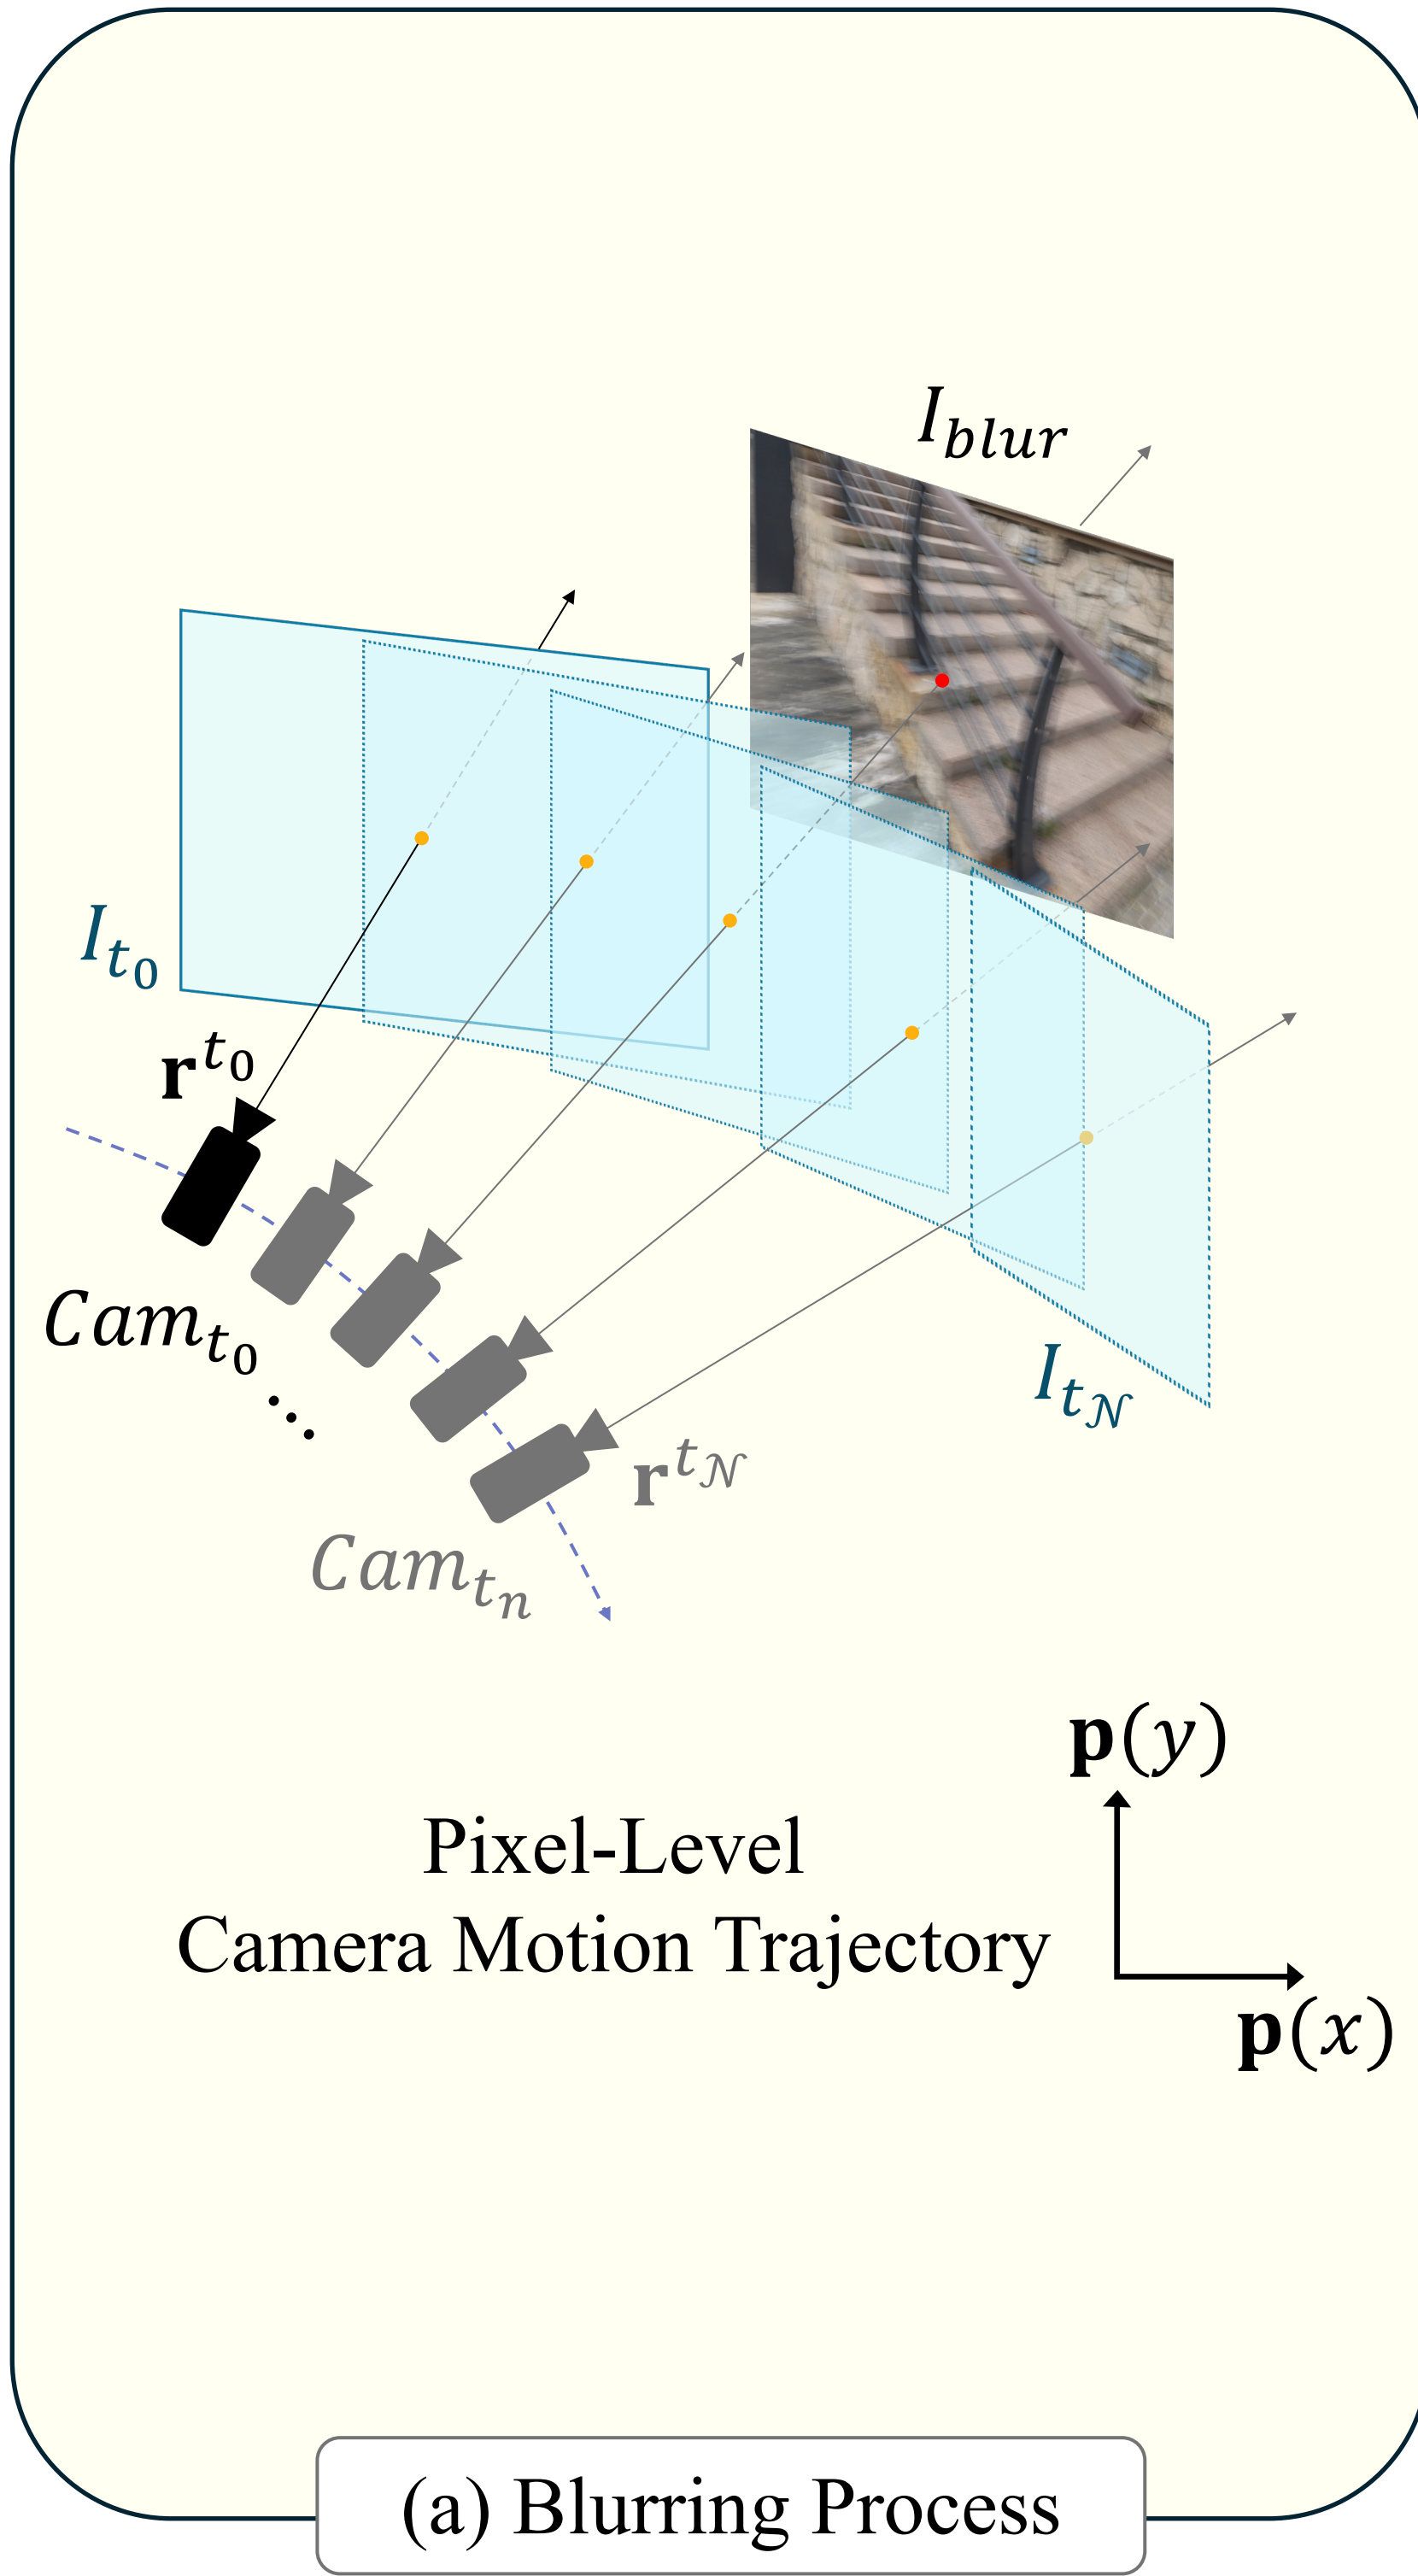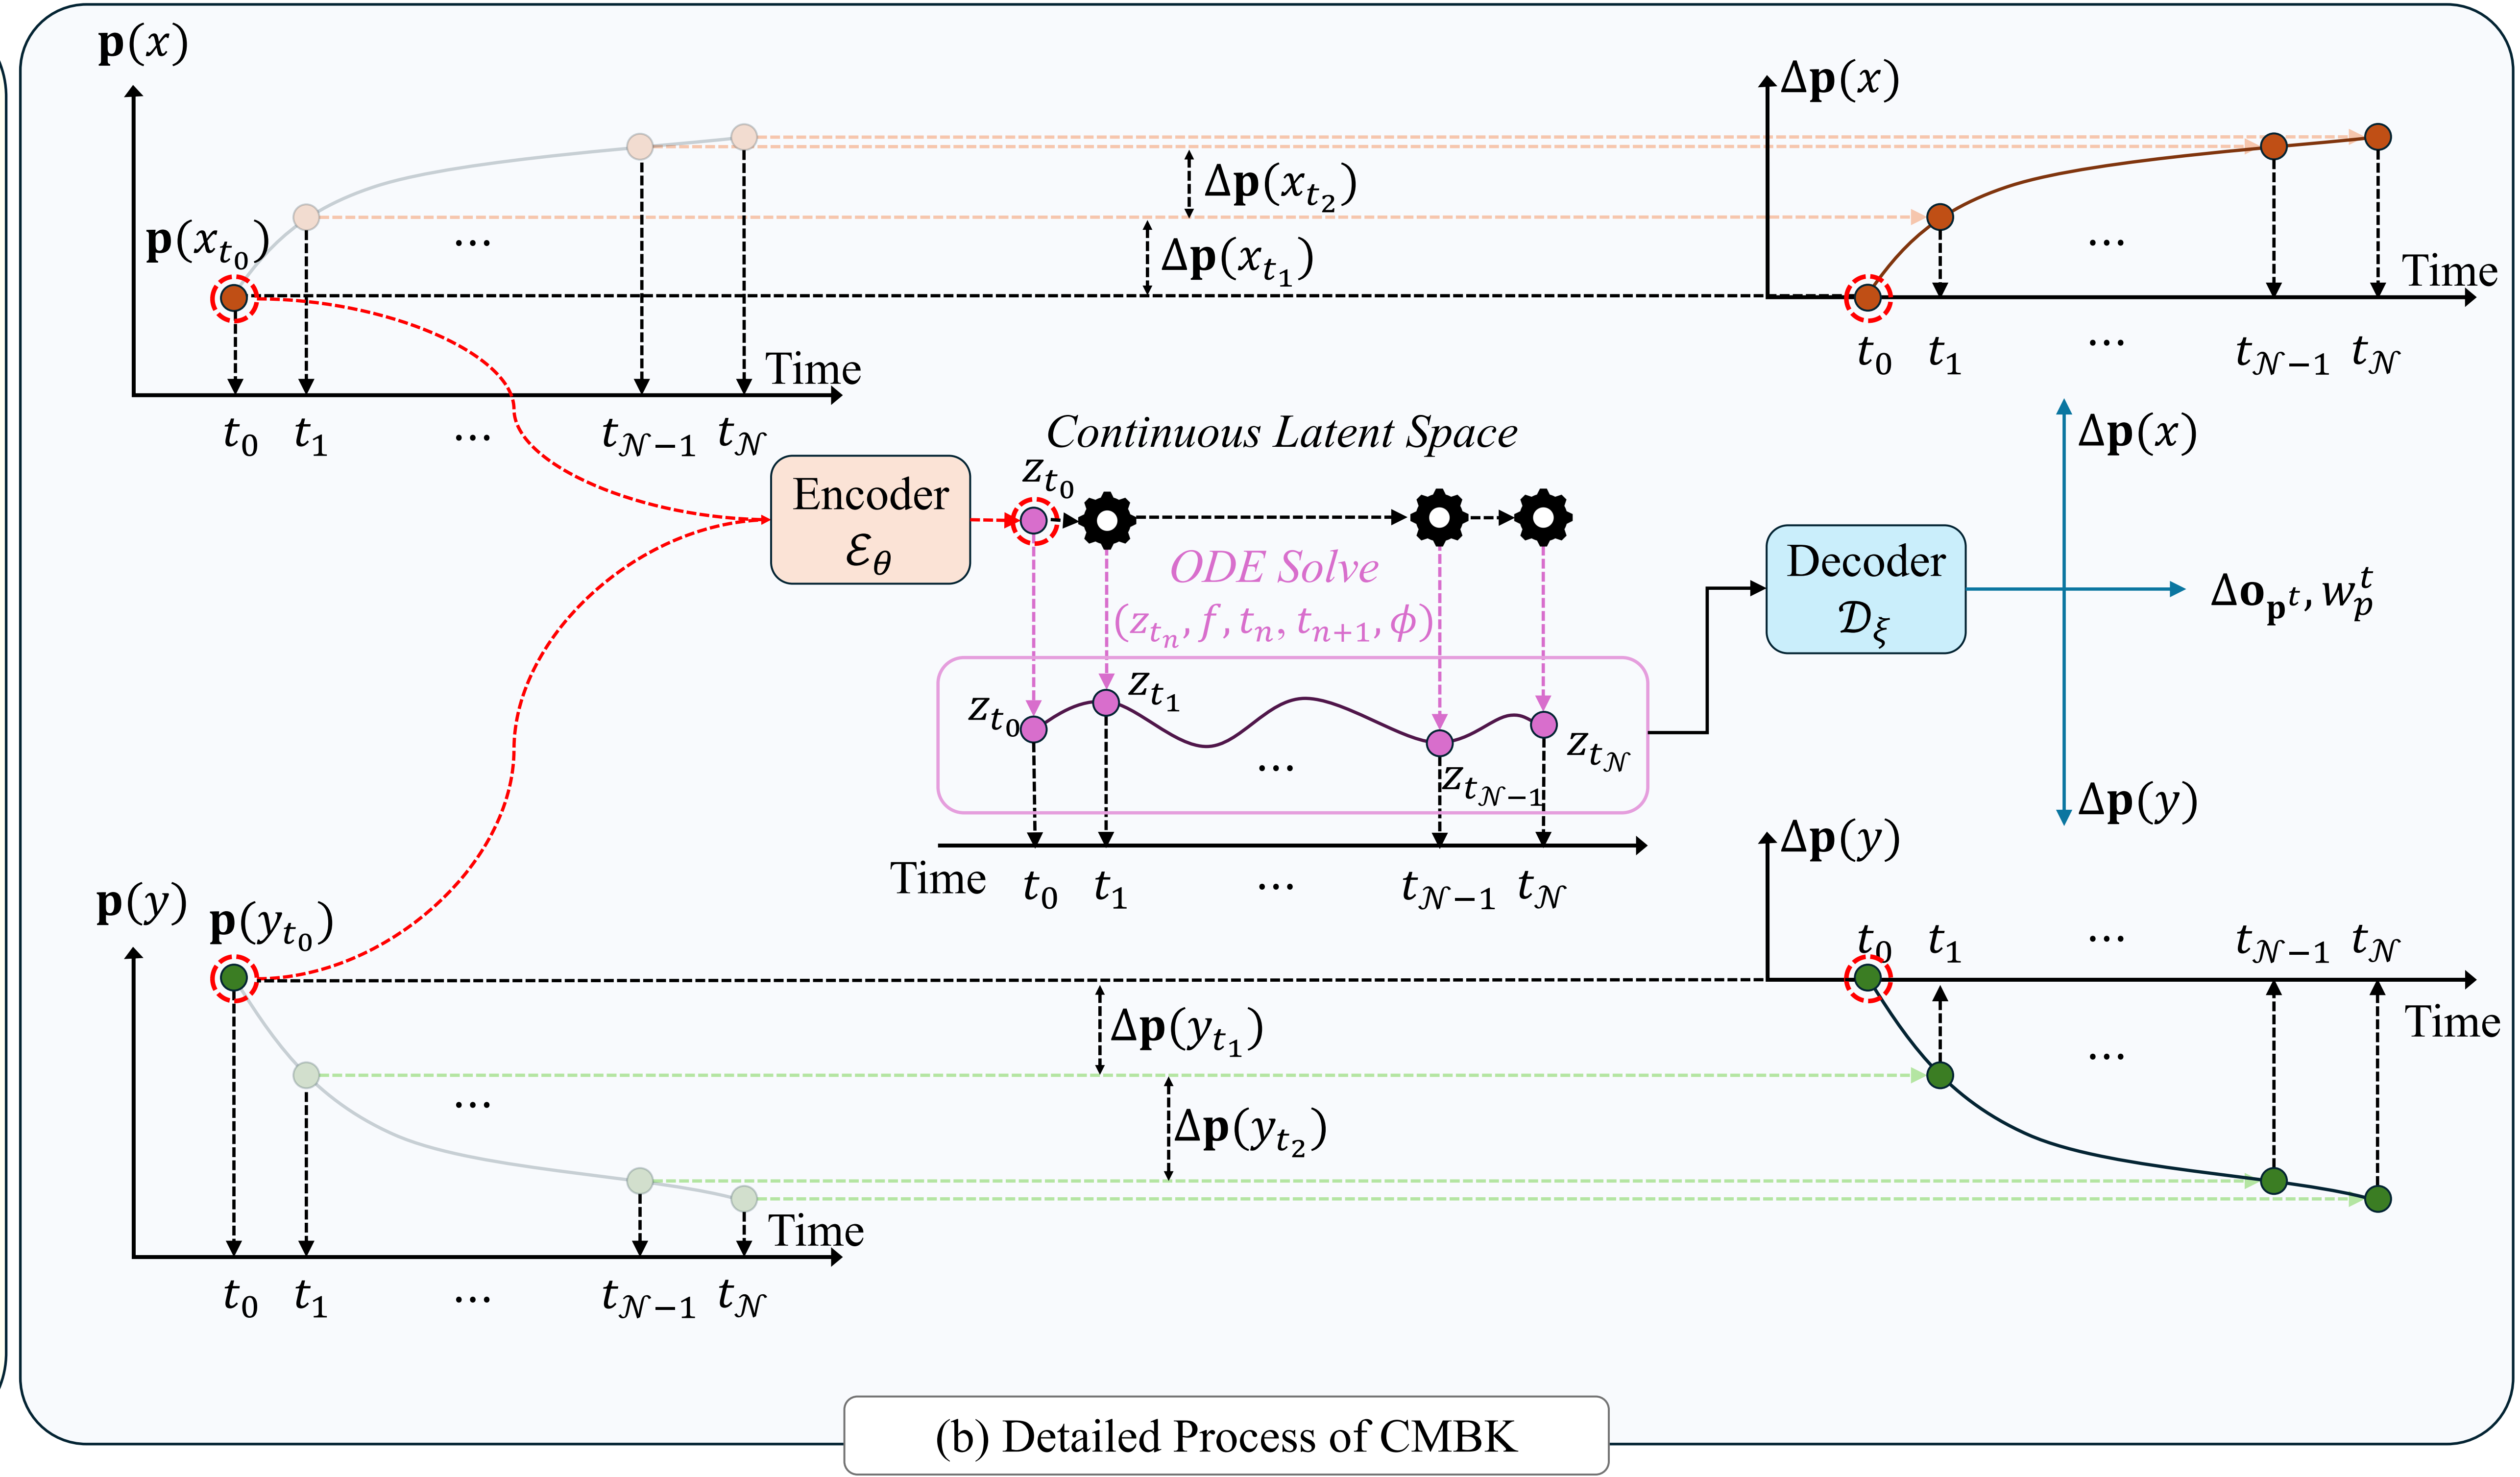

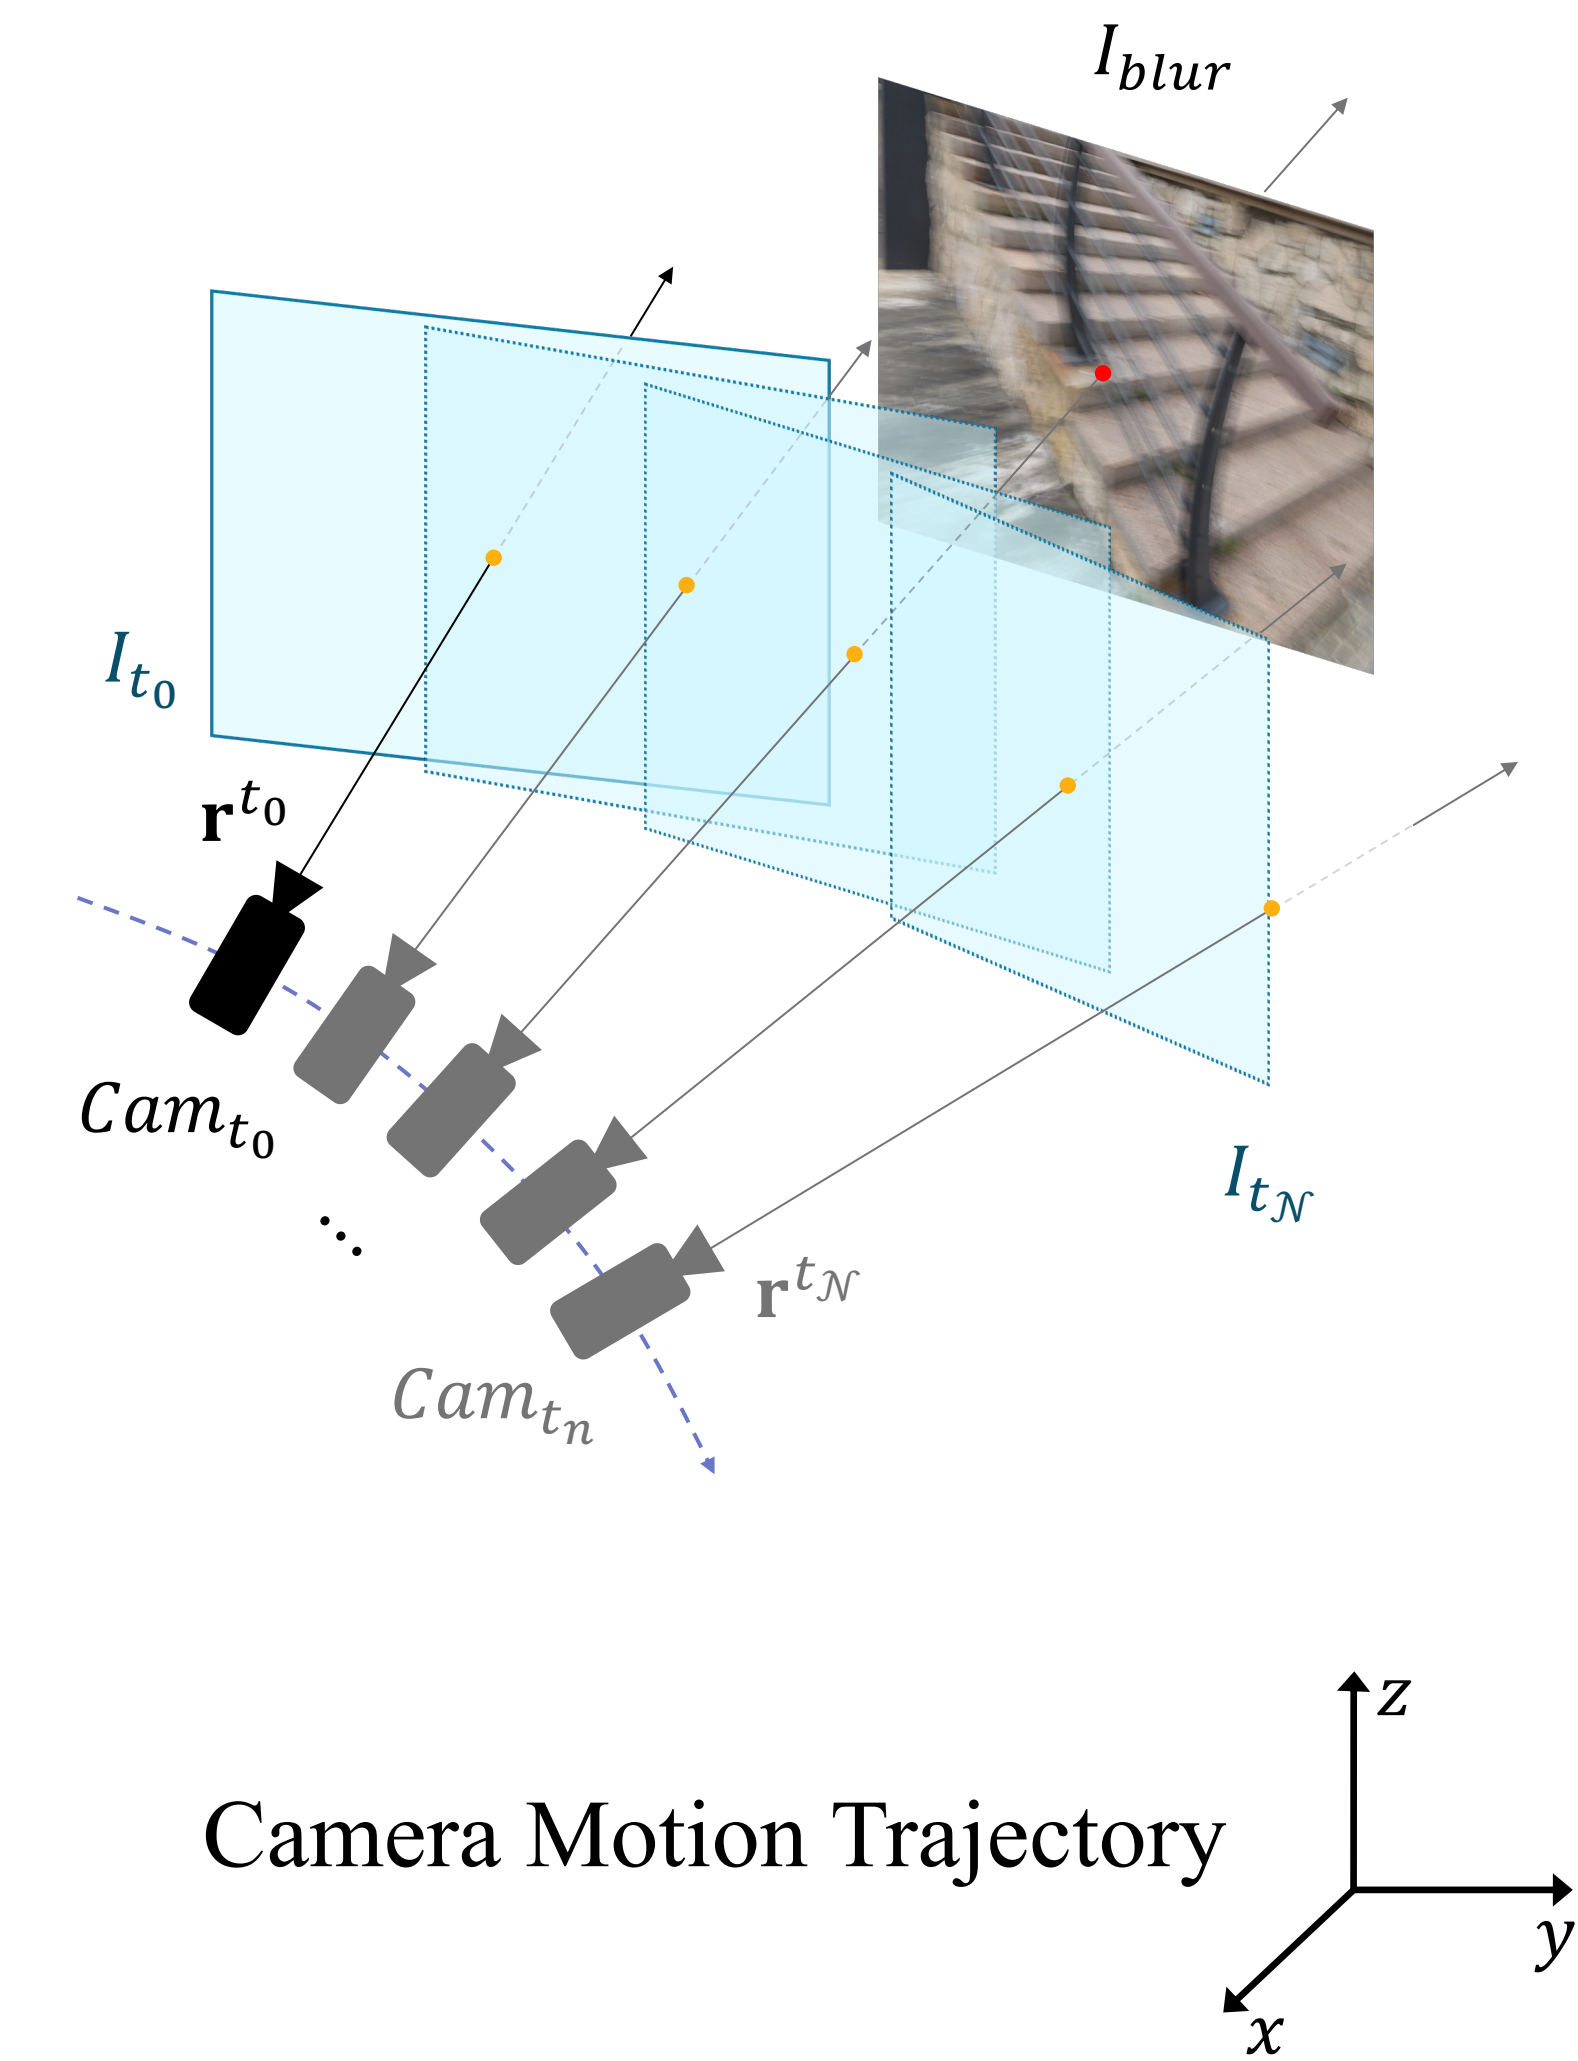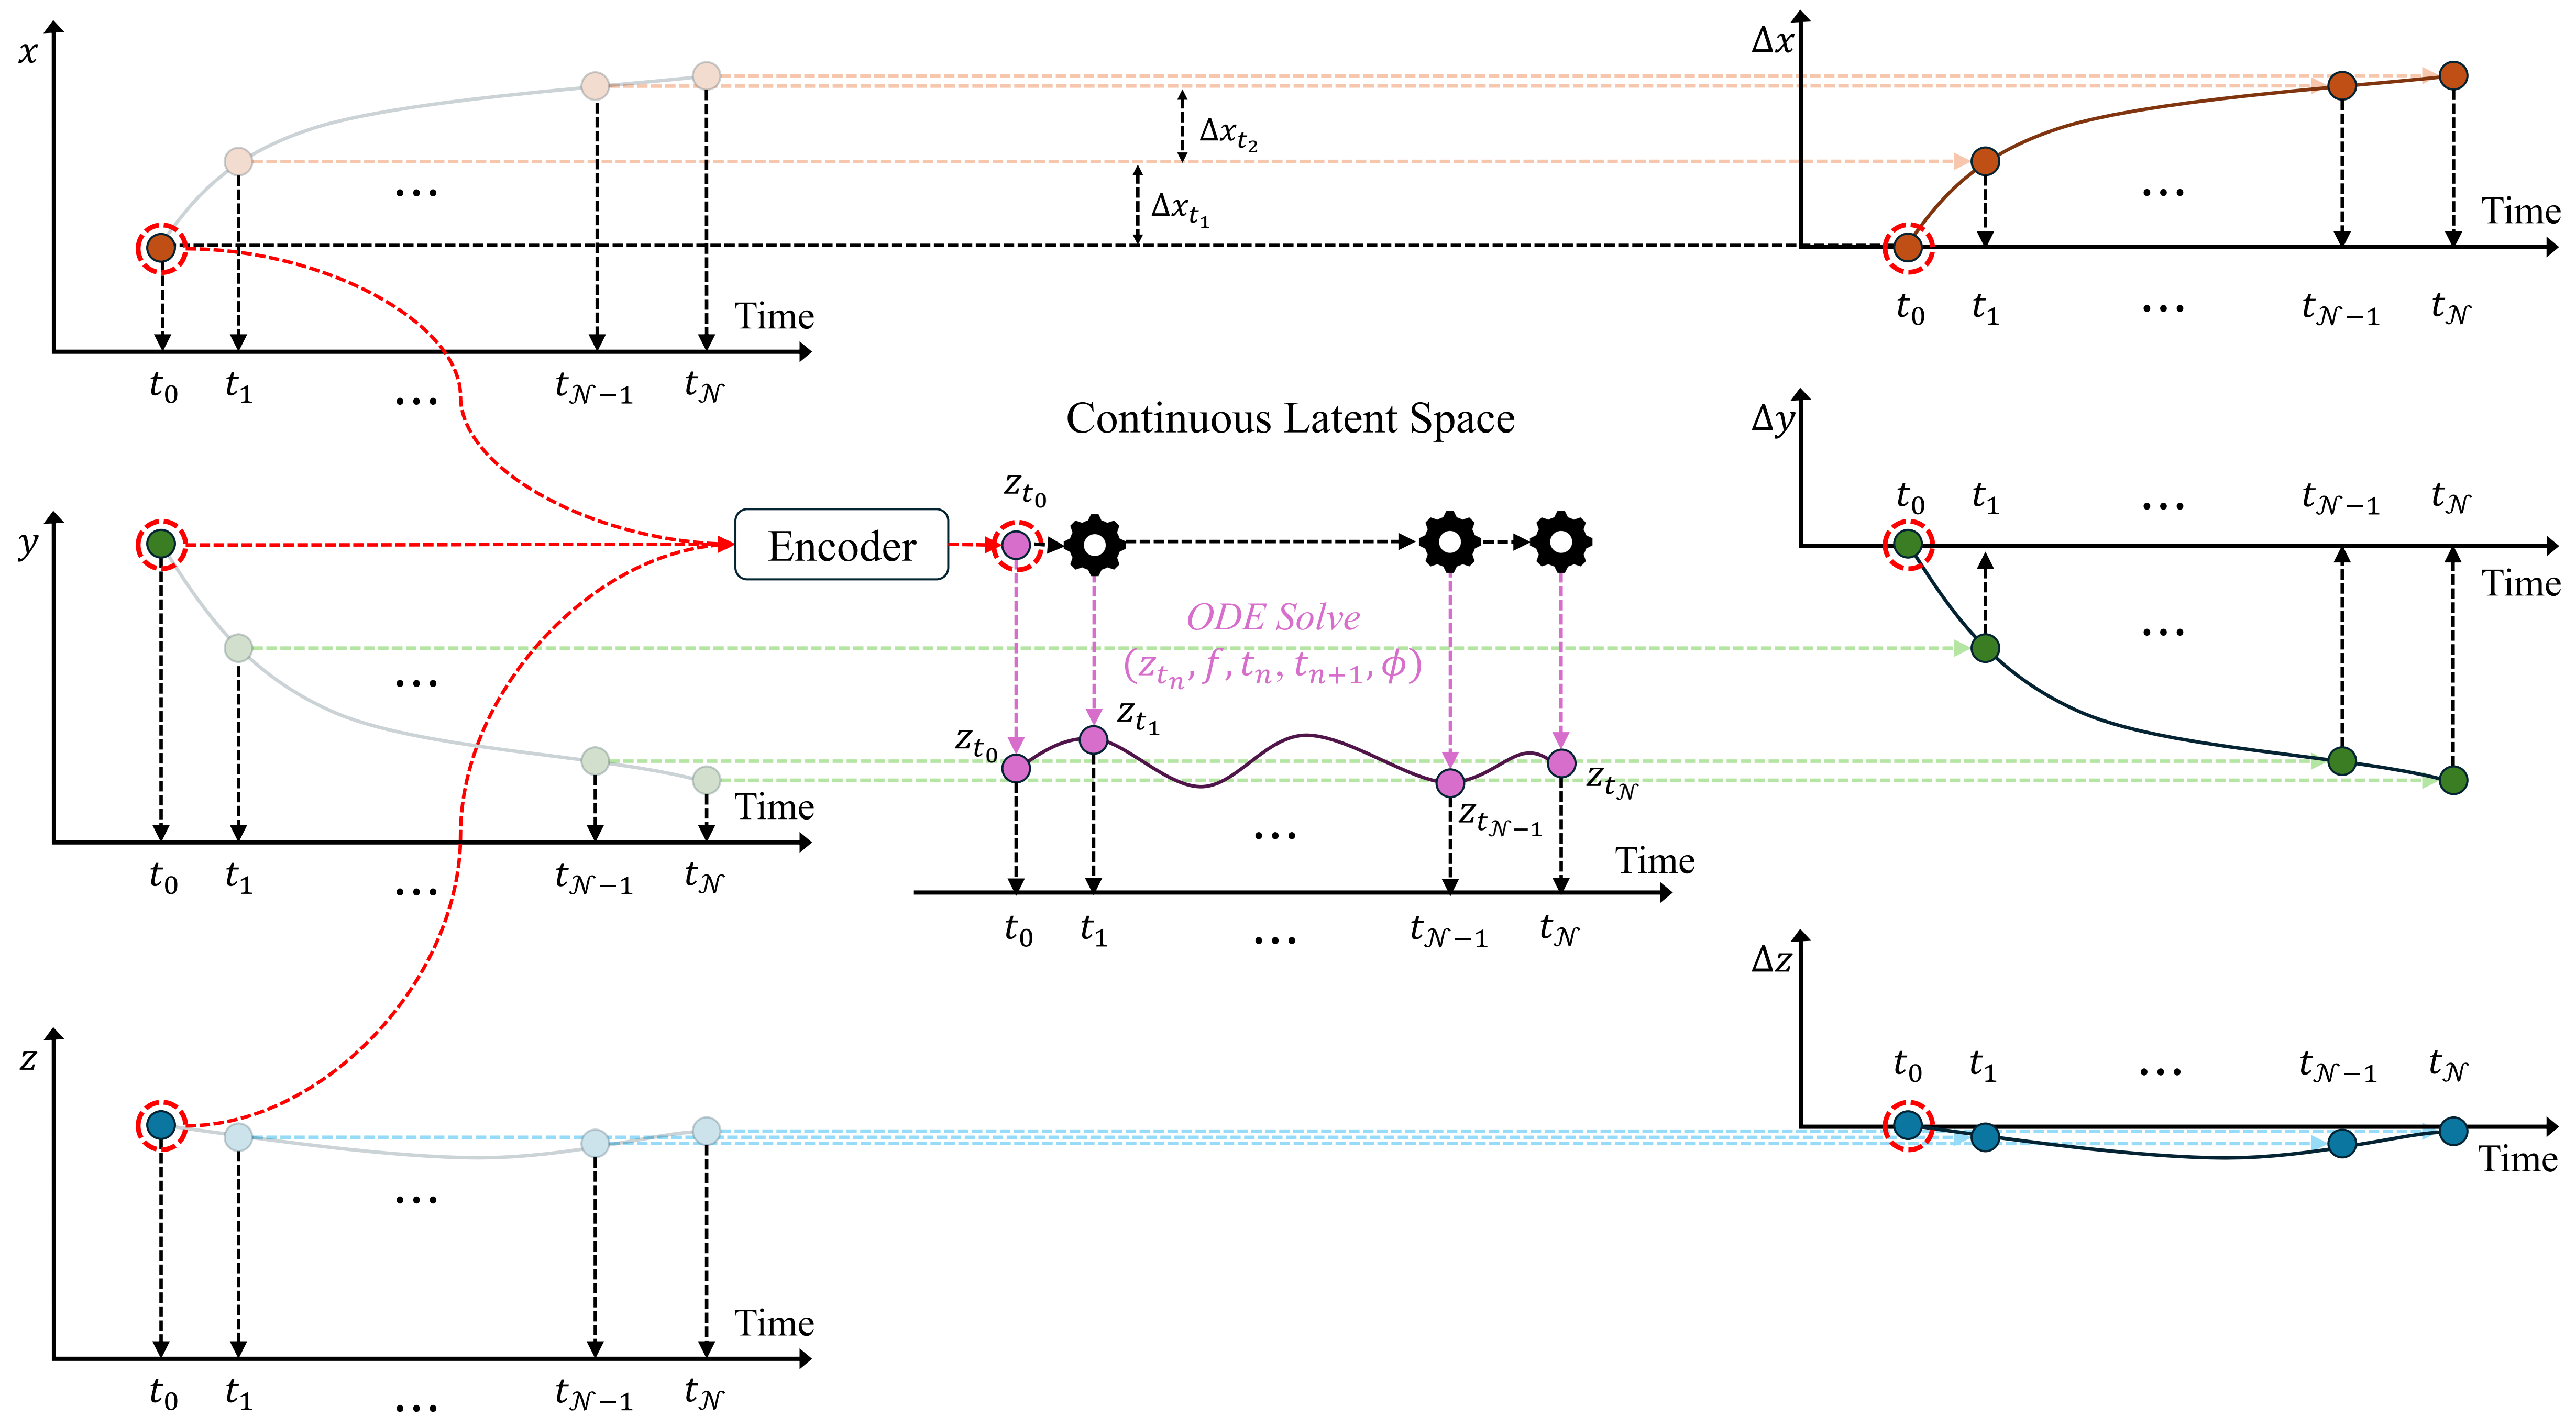

Supplement: Supplementary file 2 [file smurf_figure_appendix_1.pdf]
